# Supplementary material for: A Mountaineering Strategy to Excited States: Highly-Accurate Energies and Benchmarks for Medium Size Molecules
Source: arXiv:1912.04173 source file (2020-01-31)
Supplement: Supplementary file 1 [file FCI2-SI.pdf]

# A Mountaineering Strategy to Excited States: Highly-Accurate Energies and Benchmarks for Medium Size Molecules
# Supporting Information

Pierre-François Loos,[*,†] Filippo Lipparini,[*,‡] Martial Boggio-Pasqua,[†] Anthony Scemama,[†] and Denis Jacquemin[*,¶]

†*Laboratoire de Chimie et Physique Quantiques, CNRS et Université Toulouse III - Paul Sabatier, 118 route de Narbonne, 31062 Toulouse, France*

‡*Dipartimento di Chimica e Chimica Industriale, University of Pisa, Via Moruzzi 3, 56124 Pisa, Italy*

¶*Laboratoire CEISAM - UMR CNRS 6230, Université de Nantes, 2 Rue de la Houssinière, BP 92208, 44322 Nantes Cedex 3, France*

E-mail: loos@irsamc.ups-tlse.fr; filippo.lipparini@unipi.it; Denis.Jacquemin@univ-nantes.fr

# S1 Basis set and frozen-core effects

## S1.1 Cyanoacetylene, cyanogen, and diacetylene

Table S1: CC3 vertical transition energies of cyanoacetylene, cyanogen, and diacetylene using various atomic basis sets. FC stands for frozen core. All values are in eV.

| | 6-31+G(d) | *aug*-cc-pVDZ | *aug*-cc-pVTZ | *aug*-cc-pVQZ | | d-*aug*-cc-pVQZ | | *aug*-cc-pV5Z |
|---|---|---|---|---|---|---|---|---|
| | FC | FC | FC | FC | Full | FC | Full | FC |
| | Cyanoacetylene | | | | | | | |
| $^1\Sigma^-$ | 6.02 | 5.92 | 5.80 | 5.79 | 5.79 | 5.79 | 5.79 | 5.79 |
| $^1\Delta$ | 6.29 | 6.17 | 6.08 | 6.06 | 6.07 | 6.06 | 6.07 | 6.06 |
| $^3\Sigma^+$ | 4.44 | 4.43 | 4.45 | 4.46 | 4.46 | 4.46 | 4.46 | 4.47 |
| $^3\Delta$ | 5.35 | 5.28 | 5.22 | 5.22 | 5.21 | 5.22 | 5.21 | 5.22 |
| $^1A''$[F] | 3.70 | 3.60 | 3.54 | 3.54 | 3.54 | | | |
| | Cyanogen | | | | | | | |
| $^1\Sigma_u^-$ | 6.62 | 6.52 | 6.39 | 6.38 | 6.38 | 6.38 | 6.38 | 6.38 |
| $^1\Delta_u$ | 6.88 | 6.77 | 6.66 | 6.64 | 6.65 | 6.64 | 6.65 | 6.64 |
| $^3\Sigma_u^+$ | 4.92 | 4.89 | 4.90 | 4.91 | 4.91 | 4.91 | 4.91 | 4.92 |
| $^1\Sigma_u^-$[F] | 5.27 | 5.19 | 5.06 | 5.05 | 5.05 | 5.05 | 5.05 | 5.04 |
| | Diacetylene | | | | | | | |
| $^1\Sigma_u^-$ | 5.57 | 5.44 | 5.34 | 5.33 | 5.34 | 5.33 | 5.34 | 5.33 |
| $^1\Delta_u$ | 5.83 | 5.69 | 5.61 | 5.60 | 5.60 | 5.60 | 5.60 | 5.60 |
| $^3\Sigma_u^+$ | 4.07 | 4.06 | 4.08 | 4.10 | 4.09 | 4.10 | 4.09 | 4.11 |
| $^3\Delta_u$ | 4.93 | 4.86 | 4.80 | 4.80 | 4.80 | 4.80 | 4.80 | 4.80 |

## S1.2 Cyclopropenone, cyclopropenethione, and methylenecyclopropene

Table S2: CC3 vertical transition energies of cyclopropenone, cyclopropenethione, and methylenecyclopropene using various atomic basis sets. FC stands for frozen core. All values are in eV.

| | 6-31+G(d) | *aug*-cc-pVDZ | *aug*-cc-pVTZ | *aug*-cc-pVQZ | | d-*aug*-cc-pVQZ | *aug*-cc-pV5Z |
|---|---|---|---|---|---|---|---|
| | FC | FC | FC | FC | Full | FC | FC |
| | Cyclopropenone | | | | | | |
| $^1B_1(n \to \pi^\star)$ | 4.32 | 4.22 | 4.21 | 4.23 | 4.22 | 4.23 | 4.23 |
| $^1A_2(n \to \pi^\star)$ | 5.68 | 5.59 | 5.57 | 5.58 | 5.57 | 5.58 | 5.58 |
| $^1B_2(n \to 3s)$ | 6.39 | 6.21 | 6.32 | 6.37 | 6.38 | 6.36 | 6.38 |
| $^1B_2(\pi \to \pi^\star)$ | 6.70 | 6.56 | 6.54 | 6.56 | 6.56 | 6.56 | 6.56 |
| $^1B_2(n \to 3p)$ | 6.92 | 6.88 | 6.96 | 6.99 | 7.00 | 6.96 | 6.99 |
| $^1A_1(n \to 3p)$ | 7.00 | 6.88 | 7.00 | 7.05 | 7.06 | 7.03 | 7.06 |
| $^1A_1(\pi \to \pi^\star)$ | 8.51 | 8.32 | 8.28 | 8.28 | 8.28 | 8.22 | 8.26 |
| $^3B_1(n \to \pi^\star)$ | 4.02 | 3.90 | 3.91 | 3.93 | 3.92 | 3.93 | 3.94 |
| $^3B_2(\pi \to \pi^\star)$ | 4.92 | 4.90 | 4.89 | 4.91 | 4.90 | 4.91 | 4.92 |
| $^3A_2(n \to \pi^\star)$ | 5.48 | 5.38 | 5.37 | 5.39 | 5.37 | 5.39 | 5.39 |
| $^3A_1(\pi \to \pi^\star)$ | 6.89 | 6.79 | 6.83 | 6.84 | 6.83 | 6.84 | 6.85 |
| | Cyclopropenethione | | | | | | |
| $^1A_2(n \to \pi^\star)$ | 3.46 | 3.47 | 3.43 | 3.44 | 3.42 | 3.44 | 3.43 |
| $^1B_1(n \to \pi^\star)$ | 3.45 | 3.42 | 3.43 | 3.45 | 3.43 | 3.45 | 3.46 |
| $^1B_2(\pi \to \pi^\star)$ | 4.67 | 4.66 | 4.64 | 4.66 | 4.64 | 4.66 | 4.66 |
| $^1B_2(n \to 3s)$ | 5.26 | 5.23 | 5.34 | 5.39 | 5.39 | 5.38 | 5.40 |
| $^1A_1(\pi \to \pi^\star)$ | 5.53 | 5.52 | 5.49 | 5.49 | 5.48 | 5.49 | 5.49 |
| $^1B_2(n \to 3p)$ | 5.83 | 5.86 | 5.93 | 5.95 | 5.95 | 5.91 | 5.95 |
| $^3A_2(n \to \pi^\star)$ | 3.33 | 3.34 | 3.31 | 3.31 | 3.29 | 3.31 | 3.31 |
| $^3B_1(n \to \pi^\star)$ | 3.34 | 3.30 | 3.31 | 3.34 | 3.32 | 3.34 | 3.35 |
| $^3B_2(\pi \to \pi^\star)$ | 4.01 | 4.03 | 4.02 | 4.04 | 4.03 | 4.04 | 4.05 |
| $^3A_1(\pi \to \pi^\star)$ | 4.06 | 4.09 | 4.03 | 4.04 | 4.02 | 4.04 | 4.03 |
| | Methylenecyclopropene | | | | | | |
| $^1B_2(\pi \to \pi^\star)$ | 4.38 | 4.32 | 4.31 | 4.31 | 4.31 | 4.31 | 4.32 |
| $^1B_1(\pi \to 3s)$ | 5.65 | 5.35 | 5.44 | 5.47 | 5.48 | 5.46 | 5.47 |
| $^1A_2(\pi \to 3p)$ | 5.97 | 5.86 | 5.95 | 5.98 | 5.99 | 5.96 | 5.97 |
| $^1A_1(\pi \to \pi^\star)$ | 6.17 | 6.15 | 6.13 | 6.09 | 6.10 | 5.98 | 6.04 |
| $^3B_2(\pi \to \pi^\star)$ | 3.50 | 3.49 | 3.50 | 3.50 | 3.50 | 3.50 | 3.51 |
| $^3A_1(\pi \to \pi^\star)$ | 4.74 | 4.74 | 4.74 | 4.75 | 4.74 | 4.74 | 4.75 |

## S1.3 Acrolein, butadiene, and glyoxal

Table S3: CC3 vertical transition energies of acrolein, butadiene, and glyoxal using various atomic basis sets. FC stands for frozen core. All values are in eV.

| | 6-31+G(d) | *aug*-cc-pVDZ | *aug*-cc-pVTZ | *aug*-cc-pVQZ | | d-*aug*-cc-pVQZ | *aug*-cc-pV5Z |
|---|---|---|---|---|---|---|---|
| | FC | FC | FC | FC | Full | FC | FC |
| | | | Acrolein | | | | |
| $^1A''(n \to \pi^\star)$ | 3.83 | 3.77 | 3.74 | 3.75 | 3.74 | | |
| $^1A'(\pi \to \pi^\star)$ | 6.83 | 6.67 | 6.65 | 6.65 | 6.65 | | |
| $^1A''(n \to \pi^\star)$ | 6.94 | 6.75 | 6.75 | 6.77 | 6.76 | | |
| $^1A'(n \to 3s)$ | 7.22 | 6.99 | 7.07 | 7.11 | 7.11 | | |
| $^3A''(n \to \pi^\star)$ | 3.55 | 3.47 | 3.46 | 3.47 | 3.46 | | |
| $^3A'(\pi \to \pi^\star)$ | 3.94 | 3.95 | 3.94 | 3.95 | 3.94 | | |
| $^3A'(\pi \to \pi^\star)$ | 6.25 | 6.22 | 6.19 | 6.20 | 6.19 | | |
| $^3A''(n \to \pi^\star)$ | 6.81 | 6.60 | 6.61 | 6.63 | 6.62 | | |
| | | | Butadiene | | | | |
| $^1B_u(\pi \to \pi^\star)$ | 6.41 | 6.25 | 6.22 | 6.21 | 6.22 | | |
| $^1B_g(\pi \to 3s)$ | 6.53 | 6.26 | 6.33 | 6.35 | 6.36 | | |
| $^1A_g(\pi \to \pi^\star)$ | 6.73 | 6.68 | 6.67 | 6.67 | 6.67 | 6.67 | |
| $^1A_u(\pi \to 3p)$ | 6.87 | 6.57 | 6.64 | 6.66 | 6.67 | | |
| $^1A_u(\pi \to 3p)$ | 6.93 | 6.73 | 6.80 | 6.82 | 6.83 | | |
| $^1B_u(\pi \to 3p)$ | 7.98 | 7.86 | 7.68 | 7.54 | 7.55 | | |
| $^3B_u(\pi \to \pi^\star)$ | 3.35 | 3.36 | 3.36 | 3.37 | 3.36 | | |
| $^3A_g(\pi \to \pi^\star)$ | 5.22 | 5.21 | 5.20 | 5.21 | 5.20 | | |
| $^3B_g(\pi \to 3s)$ | 6.46 | 6.20 | 6.28 | 6.30 | 6.31 | | |
| | | | Glyoxal | | | | |
| $^1A_u(n \to \pi^\star)$ | 2.94 | 2.90 | 2.88 | 2.88 | 2.87 | 2.88 | 2.88 |
| $^1B_g(n \to \pi^\star)$ | 4.34 | 4.30 | 4.27 | 4.27 | 4.27 | 4.27 | 4.28 |
| $^1A_g(n, n \to \pi^\star, \pi^\star)$ | 6.74 | 6.70 | 6.76 | 6.76 | 6.74 | 6.76 | 6.75 |
| $^1B_g(n \to \pi^\star)$ | 6.81 | 6.59 | 6.58 | 6.59 | 6.58 | 6.58 | 6.59 |
| $^1B_u(n \to 3p)$ | 7.72 | 7.55 | 7.67 | 7.72 | 7.73 | 7.72 | 7.74 |
| $^3A_u(n \to \pi^\star)$ | 2.55 | 2.49 | 2.49 | 2.49 | 2.49 | 2.49 | 2.50 |
| $^3B_g(n \to \pi^\star)$ | 3.97 | 3.91 | 3.90 | 3.91 | 3.90 | 3.91 | 3.92 |
| $^3B_u(\pi \to \pi^\star)$ | 5.22 | 5.20 | 5.17 | 5.18 | 5.17 | 5.18 | 5.19 |
| $^3A_g(\pi \to \pi^\star)$ | 6.35 | 6.34 | 6.30 | 6.31 | 6.30 | 6.31 | 6.31 |

## S1.4 Acetone, cyanoformaldehyde, isobutene, propynal, thioacetone, and thiopropynal

Table S4: CC3 vertical transition energies of acetone, cyanoformaldehyde, isobutene, propynal, thioacetone, and thiopropynal using various atomic basis sets. FC stands for frozen core. All values are in eV.

| | 6-31+G(d) | *aug*-cc-pVDZ | *aug*-cc-pVTZ | *aug*-cc-pVQZ | | d-*aug*-cc-pVQZ |
|---|---|---|---|---|---|---|
| | FC | FC | FC | FC | Full | FC |
| | | | Acetone | | | |
| $^1A_2(n \rightarrow \pi^\star)$ | 4.55 | 4.50 | 4.48 | 4.49 | 4.48 | |
| $^1B_2(n \rightarrow 3s)$ | 6.65 | 6.31 | 6.43 | 6.48 | 6.49 | |
| $^1A_2(n \rightarrow 3p)$ | 7.83 | 7.37 | 7.45 | 7.48 | 7.49 | |
| $^1A_1(n \rightarrow 3p)$ | 7.81 | 7.39 | 7.48 | 7.52 | 7.53 | |
| $^1B_2(n \rightarrow 3p)$ | 7.87 | 7.56 | 7.59 | 7.60 | 7.61 | |
| $^3A_2(n \rightarrow \pi^\star)$ | 4.21 | 4.16 | 4.15 | 4.17 | 4.16 | |
| $^3A_1(\pi \rightarrow \pi^\star)$ | 6.32 | 6.31 | 6.28 | 6.30 | 6.28 | |
| | | | Cyanoformaldehyde | | | |
| $^1A''(n \rightarrow \pi^\star)$ | 3.91 | 3.86 | 3.83 | 3.84 | 3.83 | 3.84 |
| $^1A''(\pi \rightarrow \pi^\star)$ | 6.64 | 6.51 | 6.42 | 6.41 | 6.41 | 6.41 |
| $^3A''(n \rightarrow \pi^\star)$ | 3.53 | 3.47 | 3.46 | 3.47 | 3.46 | 3.47 |
| $^3A'(\pi \rightarrow \pi^\star)$ | 5.07 | 5.03 | 5.01 | 5.02 | 5.01 | 5.02 |
| | | | Isobutene | | | |
| $^1B_1(\pi \rightarrow 3s)$ | 6.77 | 6.39 | 6.45 | 6.47 | 6.49 | |
| $^1A_1(\pi \rightarrow 3p)$ | 7.16 | 7.00 | 7.00 | 6.99 | 7.00 | |
| $^3A_1(\pi \rightarrow \pi^\star)$ | 4.52 | 4.54 | 4.53 | 4.54 | 4.54 | |
| | | | Propynal | | | |
| $^1A''(n \rightarrow \pi^\star)$ | 3.90 | 3.85 | 3.82 | 3.83 | 3.82 | 3.83 |
| $^1A''(\pi \rightarrow \pi^\star)$ | 5.69 | 5.59 | 5.51 | 5.50 | 5.50 | 5.50 |
| $^3A''(n \rightarrow \pi^\star)$ | 3.56 | 3.50 | 3.49 | 3.50 | 3.49 | 3.50 |
| $^3A'(\pi \rightarrow \pi^\star)$ | 4.46 | 4.40 | 4.43 | 4.44 | 4.43 | 4.44 |
| | | | Thioacetone | | | |
| $^1A_2(n \rightarrow \pi^\star)$ | 2.58 | 2.59 | 2.55 | 2.56 | | |
| $^1B_2(n \rightarrow 4s)$ | 5.65 | 5.44 | 5.55 | 5.60 | | |
| $^1A_1(\pi \rightarrow \pi^\star)$ | 6.09 | 5.97 | 5.90 | 5.88 | 5.87 | |
| $^1B_2(n \rightarrow 4p)$ | 6.59 | 6.45 | 6.51 | 6.52 | | |
| $^1A_1(n \rightarrow 4p)$ | 6.95 | 6.54 | 6.61 | 6.64 | 6.64 | |
| $^3A_2(n \rightarrow \pi^\star)$ | 2.36 | 2.36 | 2.34 | 2.35 | | |
| $^3A_1(\pi \rightarrow \pi^\star)$ | 3.45 | 3.51 | 3.46 | 3.47 | 3.46 | |
| | | | Thiopropynal | | | |
| $^1A''(n \rightarrow \pi^\star)$ | 2.09 | 2.09 | 2.05 | 2.06 | 2.04 | |
| $^3A''(n \rightarrow \pi^\star)$ | 1.84 | 1.83 | 1.81 | 1.82 | 1.81 | |

## S1.5 Cyclopentadiene, furan, imidazole, pyrrole, and thiophene

Table S5: CC3 vertical transition energies of furan and pyrrole using various atomic basis sets. FC stands for frozen core. All values are in eV.

| | 6-31+G(d) | *aug*-cc-pVDZ | *aug*-cc-pVTZ | *aug*-cc-pVQZ | |
|---|---|---|---|---|---|
| | FC | FC | FC | FC | Full |
| | | | Furan | | |
| $^1A_2(\pi \rightarrow 3s)$ | 6.26 | 6.00 | 6.08 | 6.10 | 6.12 |
| $^1B_2(\pi \rightarrow \pi^\star)$ | 6.50 | 6.37 | 6.34 | 6.34 | 6.34 |
| $^1A_1(\pi \rightarrow \pi^\star)$ | 6.71 | 6.62 | 6.58 | 6.58 | 6.58 |
| $^1B_1(\pi \rightarrow 3p)$ | 6.76 | 6.55 | 6.63 | 6.65 | 6.67 |
| $^1A_2(\pi \rightarrow 3p)$ | 6.97 | 6.73 | 6.80 | 6.82 | 6.83 |
| $^1B_2(\pi \rightarrow 3p)$ | 7.53 | 7.39 | 7.23 | 7.13 | 7.14 |
| $^3B_2(\pi \rightarrow \pi^\star)$ | 4.28 | 4.25 | 4.22 | 4.22 | 4.22 |
| $^3A_1(\pi \rightarrow \pi^\star)$ | 5.56 | 5.51 | 5.48 | 5.49 | 5.48 |
| $^3A_2(\pi \rightarrow 3s)$ | 6.18 | 5.94 | 6.02 | 6.05 | 6.07 |
| $^3B_1(\pi \rightarrow 3p)$ | 6.69 | 6.51 | 6.59 | 6.61 | 6.63 |
| | | | Pyrrole | | |
| $^1A_2(\pi \rightarrow 3s)$ | 5.25 | 5.15 | 5.24 | 5.27 | 5.28 |
| $^1B_1(\pi \rightarrow 3p)$ | 5.99 | 5.89 | 5.98 | 6.01 | 6.02 |
| $^1A_2(\pi \rightarrow 3p)$ | 6.27 | 5.94 | 6.01 | 6.03 | 6.05 |
| $^1B_2(\pi \rightarrow \pi^\star)$ | 6.33 | 6.28 | 6.25 | 6.22 | 6.23 |
| $^1A_1(\pi \rightarrow \pi^\star)$ | 6.43 | 6.35 | 6.32 | 6.31 | 6.31 |
| $^1B_2(\pi \rightarrow 3p)$ | 7.20 | 7.00 | 6.83 | 6.74 | 6.75 |
| $^3B_2(\pi \rightarrow \pi^\star)$ | 4.59 | 4.56 | 4.53 | 4.53 | 4.52 |
| $^3A_2(\pi \rightarrow 3s)$ | 5.22 | 5.12 | 5.21 | 5.24 | 5.26 |
| $^3A_1(\pi \rightarrow \pi^\star)$ | 5.54 | 5.49 | 5.46 | 5.47 | 5.46 |
| $^3B_1(\pi \rightarrow 3p)$ | 5.91 | 5.82 | 5.92 | 5.95 | 5.97 |

Table S6: CC3 vertical transition energies of cyclopentadiene, imidazole, and thiophene using various atomic basis sets. FC stands for frozen core. All values are in eV.

| | 6-31+G(d) FC | *aug*-cc-pVDZ FC | *aug*-cc-pVTZ FC | *aug*-cc-pVQZ FC |
|---|---|---|---|---|
| | | Cyclopentadiene | | |
| $^1B_2(\pi \to \pi^\star)$ | 5.79 | 5.59 | 5.54 | 5.53 |
| $^1A_2(\pi \to 3s)$ | 6.08 | 5.70 | 5.77 | 5.79 |
| $^1B_1(\pi \to 3p)$ | 6.57 | 6.34 | 6.40 | 6.42 |
| $^1A_2(\pi \to 3p)$ | 6.67 | 6.39 | 6.45 | 6.46 |
| $^1B_2(\pi \to 3p)$ | 7.06 | 6.55 | 6.56 | 6.55 |
| $^1A_1(\pi \to \pi^\star)$ | 6.67 | 6.59 | 6.57 | 6.57 |
| $^3B_2(\pi \to \pi^\star)$ | 3.33 | 3.32 | 3.32 | 3.32 |
| $^3A_1(\pi \to \pi^\star)$ | 5.16 | 5.14 | 5.12 | 5.13 |
| $^3A_2(\pi \to 3s)$ | 6.01 | 5.65 | 5.73 | 5.75 |
| $^3B_1(\pi \to 3p)$ | 6.51 | 6.30 | 6.36 | 6.38 |
| | | Imidazole | | |
| $^1A''(\pi \to 3s)$ | 5.77 | 5.60 | 5.71 | 5.73 |
| $^1A'(\pi \to \pi^\star)$ | 6.51 | 6.43 | 6.41 | 6.41 |
| $^1A''(n \to \pi^\star)$ | 6.66 | 6.42 | 6.50 | 6.53 |
| $^1A'(\pi \to 3p)$ | 7.04 | 6.93 | 6.87 | 6.86 |
| $^3A'(\pi \to \pi^\star)$ | 4.83 | 4.78 | 4.75 | 4.76 |
| $^3A''(\pi \to 3s)$ | 5.72 | 5.57 | 5.67 | 5.70 |
| $^3A'(\pi \to \pi^\star)$ | 5.88 | 5.78 | 5.74 | 5.75 |
| $^3A''(n \to \pi^\star)$ | 6.48 | 6.37 | 6.33 | 6.33 |
| | | Thiophene | | |
| $^1A_1(\pi \to \pi^\star)$ | 5.79 | 5.70 | 5.65 | 5.64 |
| $^1B_2(\pi \to \pi^\star)$ | 6.23 | 6.05 | 5.96 | 5.94 |
| $^1A_2(\pi \to 3s)$ | 6.26 | 6.07 | 6.14 | 6.16 |
| $^1B_1(\pi \to 3p)$ | 6.18 | 6.19 | 6.14 | 6.11 |
| $^1A_2(\pi \to 3p)$ | 6.32 | 6.33 | 6.25 | 6.22 |
| $^1B_1(\pi \to 3s)$ | 6.62 | 6.42 | 6.50 | 6.53 |
| $^1B_2(\pi \to 3p)$ | 7.45 | 7.45 | 7.29 | 7.18 |
| $^1A_1(\pi \to \pi^\star)$ | 7.50 | 7.41 | 7.35 | 7.33 |
| $^3B_2(\pi \to \pi^\star)$ | 3.95 | 3.96 | 3.94 | 3.93 |
| $^3A_1(\pi \to \pi^\star)$ | 4.90 | 4.82 | 4.77 | 4.77 |
| $^3B_1(\pi \to 3p)$ | 6.00 | 6.01 | 5.95 | 5.92 |
| $^3A_2(\pi \to 3s)$ | 6.20 | 6.01 | 6.09 | 5.99 |

## S1.6 Benzene, pyrazine, and tetrazine

Table S7: CC3 vertical transition energies of benzene using various atomic basis sets. FC stands for frozen core. All values are in eV.

| | 6-31+G(d) FC | *aug*-cc-pVDZ FC | *aug*-cc-pVTZ FC | *aug*-cc-pVQZ FC |
|---|---|---|---|---|
| | | Benzene | | |
| $^1B_{2u}(\pi \to \pi^\star)$ | 5.13 | 5.11 | 5.09 | 5.09 |
| $^1B_{1u}(\pi \to \pi^\star)$ | 6.68 | 6.50 | 6.44 | 6.43 |
| $^1E_{1g}(\pi \to 3s)$ | 6.75 | 6.46 | 6.52 | 6.54 |
| $^1A_{2u}(\pi \to 3p)$ | 7.24 | 7.02 | 7.08 | 7.10 |
| $^1E_{2u}(\pi \to 3p)$ | 7.34 | 7.09 | 7.15 | 7.16 |
| $^3B_{1u}(\pi \to \pi^\star)$ | 4.18 | 4.19 | 4.18 | 4.19 |
| $^3E_{1u}(\pi \to \pi^\star)$ | 4.95 | 4.89 | 4.86 | 4.87 |
| $^3B_{2u}(\pi \to \pi^\star)$ | 6.06 | 5.86 | 5.81 | 5.81 |

Table S8: CC3 vertical transition energies of pyrazine and tetrazine using various atomic basis sets. FC stands for frozen core. All values are in eV.

| | 6-31+G(d) | *aug*-cc-pVDZ | *aug*-cc-pVTZ | *aug*-cc-pVQZ | |
|---|---|---|---|---|---|
| | FC | FC | FC | FC | Full |
| | | | Pyrazine | | |
| $^1B_{3u}(n \rightarrow \pi^\star)$ | 4.28 | 4.19 | 4.14 | 4.14 | |
| $^1A_u(n \rightarrow \pi^\star)$ | 5.08 | 4.98 | 4.97 | 4.98 | 4.97 |
| $^1B_{2u}(\pi \rightarrow \pi^\star)$ | 5.10 | 5.07 | 5.03 | 5.02 | 5.02 |
| $^1B_{2g}(n \rightarrow \pi^\star)$ | 5.86 | 5.78 | 5.71 | 5.7 | 1 |
| $^1A_g(n \rightarrow 3s)$ | 6.74 | 6.54 | 6.66 | 6.70 | 6.71 |
| $^1B_{1g}(n \rightarrow \pi^\star)$ | 6.87 | 6.75 | 6.73 | 6.73 | |
| $^1B_{1u}(\pi \rightarrow \pi^\star)$ | 7.10 | 6.92 | 6.86 | 6.85 | 6.85 |
| $^1B_{1g}(\pi \rightarrow 3s)$ | 7.36 | 7.13 | 7.20 | 7.23 | |
| $^1B_{2u}(n \rightarrow 3p)$ | 7.39 | 7.14 | 7.25 | 7.29 | 7.30 |
| $^1B_{1u}(n \rightarrow 3p)$ | 7.56 | 7.38 | 7.45 | 7.48 | 7.49 |
| $^1B_{1u}(\pi \rightarrow \pi^\star)$ | 8.19 | 7.99 | 7.94 | 7.93 | 7.93 |
| $^3B_{3u}(n \rightarrow \pi^\star)$ | 3.68 | 3.60 | 3.59 | 3.59 | 3.59 |
| $^3B_{1u}(\pi \rightarrow \pi^\star)$ | 4.39 | 4.40 | 4.39 | 4.40 | 4.39 |
| $^3B_{2u}(\pi \rightarrow \pi^\star)$ | 4.56 | 4.46 | 4.40 | 4.40 | 4.40 |
| $^3A_u(n \rightarrow \pi^\star)$ | 5.05 | 4.93 | 4.93 | 4.94 | |
| $^3B_{2g}(n \rightarrow \pi^\star)$ | 5.18 | 5.11 | 5.08 | 5.09 | 5.07 |
| $^3B_{1u}(\pi \rightarrow \pi^\star)$ | 5.38 | 5.32 | 5.29 | 5.29 | 5.28 |
| | | | Tetrazine | | |
| $^1B_{3u}(n \rightarrow \pi^\star)$ | 2.53 | 2.49 | 2.46 | 2.45 | 2.45 |
| $^1A_u(n \rightarrow \pi^\star)$ | 3.75 | 3.69 | 3.67 | 3.68 | 3.67 |
| $^1A_g(n, n \rightarrow \pi^\star, \pi^\star)$ | 6.22 | 6.22 | 6.21 | 6.19 | 6.17 |
| $^1B_{1g}(n \rightarrow \pi^\star)$ | 5.01 | 4.97 | 4.91 | 4.90 | 4.88 |
| $^1B_{2u}(\pi \rightarrow \pi^\star)$ | 5.29 | 5.27 | 5.23 | 5.22 | 5.21 |
| $^1B_{2g}(n \rightarrow \pi^\star)$ | 5.56 | 5.53 | 5.46 | 5.46 | 5.45 |
| $^1A_u(n \rightarrow \pi^\star)$ | 5.61 | 5.59 | 5.52 | 5.52 | 5.50 |
| $^1B_{3g}(n, n \rightarrow \pi^\star, \pi^\star)$ | 7.64 | 7.62 | 7.62 | 7.60 | 7.58 |
| $^1B_{2g}(n \rightarrow \pi^\star)$ | 6.24 | 6.17 | 6.13 | 6.13 | 6.10 |
| $^1B_{1g}(n \rightarrow \pi^\star)$ | 7.04 | 6.98 | 6.92 | 6.92 | 6.91 |
| $^3B_{3u}(n \rightarrow \pi^\star)$ | 1.87 | 1.86 | 1.85 | 1.86 | 1.85 |
| $^3A_u(n \rightarrow \pi^\star)$ | 3.48 | 3.43 | 3.44 | 3.45 | 3.43 |
| $^3B_{1g}(n \rightarrow \pi^\star)$ | 4.25 | 4.23 | 4.20 | 4.21 | 4.18 |
| $^3B_{1u}(\pi \rightarrow \pi^\star)$ | 4.54 | 4.54 | 4.54 | 4.54 | 4.53 |
| $^3B_{2u}(\pi \rightarrow \pi^\star)$ | 4.65 | 4.58 | 4.52 | 4.52 | 4.51 |
| $^3B_{2g}(n \rightarrow \pi^\star)$ | 5.11 | 5.09 | 5.05 | 5.05 | 5.04 |
| $^3A_u(n \rightarrow \pi^\star)$ | 5.17 | 5.15 | 5.11 | 5.11 | 5.10 |
| $^3B_{3g}(n, n \rightarrow \pi^\star, \pi^\star)$ | 7.35 | 7.33 | 7.35 | 7.34 | 7.32 |
| $^3B_{1u}(\pi \rightarrow \pi^\star)$ | 5.51 | 5.46 | 5.42 | 5.43 | 5.42 |

### S1.6.1 Pyridazine, pyridine, pyrimidine and triazine

Table S9: CC3 vertical transition energies of pyridazine and pyridine using various atomic basis sets. FC stands for frozen core. All values are in eV.

| | 6-31+G(d) FC | *aug*-cc-pVDZ FC | *aug*-cc-pVTZ FC | *aug*-cc-pVQZ FC |
|---|---|---|---|---|
| | Pyridazine | | | |
| $^1B_1(n \rightarrow \pi^\star)$ | 3.95 | 3.86 | 3.83 | 3.83 |
| $^1A_2(n \rightarrow \pi^\star)$ | 4.49 | 4.39 | 4.37 | 4.38 |
| $^1A_1(\pi \rightarrow \pi^\star)$ | 5.36 | 5.33 | 5.29 | 5.29 |
| $^1A_2(n \rightarrow \pi^\star)$ | 5.88 | 5.80 | 5.74 | 5.74 |
| $^1B_2(n \rightarrow 3s)$ | 6.26 | 6.06 | 6.17 | 6.21 |
| $^1B_1(n \rightarrow \pi^\star)$ | 6.51 | 6.41 | 6.37 | 6.37 |
| $^1B_2(\pi \rightarrow \pi^\star)$ | 6.96 | 6.79 | 6.74 | 6.73 |
| $^3B_1(n \rightarrow \pi^\star)$ | 3.27 | 3.20 | 3.19 | 3.20 |
| $^3A_2(n \rightarrow \pi^\star)$ | 4.19 | 4.11 | 4.11 | 4.12 |
| $^3B_2(\pi \rightarrow \pi^\star)$ | 4.39 | 4.39 | 4.38 | 4.39 |
| $^3A_1(\pi \rightarrow \pi^\star)$ | 4.93 | 4.87 | 4.83 | 4.82 |
| | Pyridine | | | |
| $^1B_1(n \rightarrow \pi^\star)$ | 5.12 | 5.01 | 4.96 | 4.96 |
| $^1B_2(\pi \rightarrow \pi^\star)$ | 5.23 | 5.21 | 5.17 | 5.17 |
| $^1A_2(n \rightarrow \pi^\star)$ | 5.55 | 5.41 | 5.40 | 5.41 |
| $^1A_1(\pi \rightarrow \pi^\star)$ | 6.84 | 6.64 | 6.63 | 6.62 |
| $^1A_1(n \rightarrow 3s)$ | 6.92 | 6.71 | 6.76 | 6.80 |
| $^1A_2(\pi \rightarrow 3s)$ | 6.98 | 6.74 | 6.81 | 6.83 |
| $^1B_2(\pi \rightarrow \pi^\star)$ | 7.50 | 7.40 | 7.38 | 7.40 |
| $^1B_1(\pi \rightarrow 3p)$ | 7.54 | 7.32 | 7.38 | 7.40 |
| $^1A_1(\pi \rightarrow \pi^\star)$ | 7.56 | 7.34 | 7.39 | 7.40 |
| $^3A_1(\pi \rightarrow \pi^\star)$ | 4.33 | 4.34 | 4.33 | 4.34 |
| $^3B_1(n \rightarrow \pi^\star)$ | 4.57 | 4.47 | 4.46 | 4.47 |
| $^3B_2(\pi \rightarrow \pi^\star)$ | 4.92 | 4.83 | 4.79 | 4.79 |
| $^3A_1(\pi \rightarrow \pi^\star)$ | 5.14 | 5.08 | 5.05 | 5.05 |
| $^3A_2(n \rightarrow \pi^\star)$ | 5.51 | 5.37 | 5.35 | 5.37 |
| $^3B_2(\pi \rightarrow \pi^\star)$ | 6.46 | 6.30 | 6.25 | 6.25 |

Table S10: CC3 vertical transition energies of pyrimidine and triazine using various atomic basis sets. FC stands for frozen core. All values are in eV.

| | 6-31+G(d) FC | *aug*-cc-pVDZ FC | *aug*-cc-pVTZ FC | *aug*-cc-pVQZ FC |
|---|---|---|---|---|
| | | Pyrimidine | | |
| $^1B_1(n \rightarrow \pi^\star)$ | 4.58 | 4.48 | 4.44 | 4.45 |
| $^1A_2(n \rightarrow \pi^\star)$ | 4.99 | 4.89 | 4.86 | 4.87 |
| $^1B_2(\pi \rightarrow \pi^\star)$ | 5.47 | 5.44 | 5.41 | 5.40 |
| $^1A_2(n \rightarrow \pi^\star)$ | 6.07 | 5.98 | 5.93 | 5.93 |
| $^1B_1(n \rightarrow \pi^\star)$ | 6.39 | 6.29 | 6.26 | 6.27 |
| $^1B_2(n \rightarrow 3s)$ | 6.81 | 6.61 | 6.72 | 6.76 |
| $^1A_1(\pi \rightarrow \pi^\star)$ | 7.08 | 6.93 | 6.87 | 6.86 |
| $^3B_1(n \rightarrow \pi^\star)$ | 4.20 | 4.12 | 4.10 | 4.11 |
| $^3A_1(\pi \rightarrow \pi^\star)$ | 4.55 | 4.56 | 4.55 | 4.56 |
| $^3A_2(n \rightarrow \pi^\star)$ | 4.77 | 4.67 | 4.66 | 4.67 |
| $^3B_2(\pi \rightarrow \pi^\star)$ | 5.08 | 5.00 | 4.96 | 4.96 |
| | | Triazine | | |
| $^1A_1''(n \rightarrow \pi^\star)$ | 4.85 | 4.76 | 4.73 | 4.74 |
| $^1A_2''(n \rightarrow \pi^\star)$ | 4.84 | 4.78 | 4.74 | 4.74 |
| $^1E''(n \rightarrow \pi^\star)$ | 4.89 | 4.82 | 4.78 | 4.79 |
| $^1A_2'(\pi \rightarrow \pi^\star)$ | 5.84 | 5.81 | 5.78 | 5.78 |
| $^1A_1'(\pi \rightarrow \pi^\star)$ | 7.45 | 7.31 | 7.24 | 7.23 |
| $^1E'(n \rightarrow 3s)$ | 7.44 | 7.24 | 7.35 | 7.39 |
| $^1E''(n \rightarrow \pi^\star)$ | 7.89 | 7.82 | 7.79 | 7.78 |
| $^1E'(\pi \rightarrow \pi^\star)$ | 8.12 | 7.97 | 7.92 | 7.92 |
| $^3A_2''(n \rightarrow \pi^\star)$ | 4.40 | 4.35 | 4.33 | 4.34 |
| $^3E''(n \rightarrow \pi^\star)$ | 4.59 | 4.52 | 4.51 | 4.51 |
| $^3A_1''(n \rightarrow \pi^\star)$ | 4.87 | 4.78 | 4.75 | 4.76 |
| $^3A_1'(\pi \rightarrow \pi^\star)$ | 4.88 | 4.88 | 4.88 | 4.89 |
| $^3E'(\pi \rightarrow \pi^\star)$ | 5.70 | 5.64 | 5.61 | 5.61 |
| $^3A_2'(\pi \rightarrow \pi^\star)$ | 6.85 | 6.69 | 6.63 | 6.62 |

# S2 Multiconfigurational results

## S2.1 Basis set effects

Table S11: Vertical transition energies of cyanoacetylene, cyanogen, and diacetylene using various atomic basis sets and multi-reference methods. All values are in eV and have been obtained within the FC approximation. The CASPT2 calculations are performed with a level shift of 0.3 and a IPEA of 0.25. Pop, AVDZ, AVTZ, and AVQZ respectively stand for 6-31+G(d), *aug*-cc-pVDZ, *aug*-cc-pVTZ, and *aug*-cc-pVQZ.

| | CASPT2(8,8) | | | | PC-NEVPT2(8,8) | | | | SC-NEVPT2(8,8) | | | |
|---|---|---|---|---|---|---|---|---|---|---|---|---|
| | Pop | AVDZ | AVTZ | AVQZ | Pop | AVDZ | AVTZ | AVQZ | Pop | AVDZ | AVTZ | AVQZ |
| | Cyanoacetylene | | | | | | | | | | | |
| $^1\Sigma^-$ | | 6.00 | 5.86 | | | 5.93 | 5.78 | | | 5.98 | 5.83 | |
| $^1\Delta$ | | 6.26 | 6.13 | | | 6.22 | 6.10 | | | 6.27 | 6.14 | |
| $^3\Sigma^+$ | | 4.47 | 4.45 | | | 4.46 | 4.45 | | | 4.51 | 4.49 | |
| $^3\Delta$ | | 5.30 | 5.21 | | | 5.28 | 5.19 | | | 5.31 | 5.23 | |
| | Cyanogen | | | | | | | | | | | |
| $^1\Sigma_u^-$ | 6.63 | 6.56 | 6.40 | 6.37 | 6.56 | 6.49 | 6.32 | 6.29 | 6.61 | 6.54 | 6.37 | 6.34 |
| $^1\Delta_u$ | 6.93 | 6.84 | 6.70 | 6.66 | 6.91 | 6.81 | 6.66 | 6.63 | 6.95 | 6.86 | 6.71 | 6.68 |
| $^3\Sigma_u^+$ | 4.91 | 4.89 | 4.86 | 4.86 | 4.92 | 4.91 | 4.88 | 4.89 | 4.96 | 4.95 | 4.92 | 4.93 |
| $^1\Sigma_u^-$[F] | | 5.23 | 5.07 | | | 5.14 | 4.97 | | | 5.17 | 5.01 | |
| | Diacetylene | | | | | | | | | | | |
| $^1\Sigma_u^-$ | | 5.56 | 5.43 | | | 5.47 | 5.33 | | | 5.53 | 5.39 | |
| $^1\Delta_u$ | | 5.80 | 5.68 | | | 5.73 | 5.61 | | | 5.78 | 5.67 | |
| $^3\Sigma_u^+$ | | 4.12 | 4.11 | | | 4.09 | 4.08 | | | 4.14 | 4.13 | |
| $^3\Delta_u$ | | 4.89 | 4.81 | | | 4.86 | 4.78 | | | 4.90 | 4.82 | |

## S2.2 Active Spaces

In the following tables, NEVPT2 vertical transition energies are provided using different sizes of active space. The composition of the active space is specified in terms of number of active orbitals per irreducible representation only for the NEVPT2 result chosen in the article (Tables 1–4). Similarly, the state-averaging procedure and the CASSCF vertical transition energies given correspond to the underlying reference calculation for the final NEVPT2 values of the article. Note that, in all these calculations, the ground state is always included in the state averaging procedure. In addition, we chose carefully the states to be averaged in the case of non-abelian point groups in order to describe correctly the degeneracy of doubly-degenerate states (e.g., $\Delta$ states of cyanoacetylene, cyanogen and diacetylene, and $E$ states of benzene and triazine).

Table S12: NEVPT2/aug-cc-pVTZ vertical transition energies (in eV) of acetone.

| State | Active space $(a_1, b_1, b_2, a_2)$ | State average $(A_1, B_1, B_2, A_2)$ | CASSCF | NEVPT2 |
|---|---|---|---|---|
| $^1A_2(\text{V}; n \to \pi^\star)$ | (2,3,1,0) | (1,0,0,2) | $4.77^b$ | $4.57^a$,$4.48^b$ |
| $^1B_2(\text{R}; n \to 3s)$ | (4,2,1,0) | (1,0,2,0) | $5.50^c$ | $6.81^c$ |
| $^1A_2(\text{R}; n \to 3p)$ | (2,3,1,0) | (1,0,0,2) | $7.46^b$ | $7.65^b$ |
| $^1A_1(\text{R}; n \to 3p)$ | (2,2,2,0) | (2,0,0,0) | $7.03^d$ | $7.75^d$ |
| $^1B_2(\text{R}; n \to 3p)$ | (4,2,1,0) | (1,0,2,0) | $6.44^c$ | $7.91^c$ |
| $^3A_2(\text{V}; n \to \pi^\star)$ | (2,2,1,0) | (1,0,0,1) | $4.47^a$ | $4.20^a$ |
| $^3A_1(\text{V}; \pi \to \pi^\star)$ | (2,2,0,0) | (2,0,0,0) | $6.22^e$ | $6.28^e$ |

[a]Using reference (6e,5o) active space including valence $\pi$, $n_\text{O}$, $\sigma_\text{CO}$ and $\sigma^*_\text{CO}$ orbitals. [b]Using reference (6e,6o) active space including valence $\pi$, $n_\text{O}$, $\sigma_\text{CO}$, $\sigma^*_\text{CO}$ and $3p_x$ orbitals. [c]Using reference (6e,7o) active space including valence $\pi$, $n_\text{O}$, $\sigma_\text{CO}$, $\sigma^*_\text{CO}$, $3s$ and $3p_z$ orbitals. [d]Using reference (6e,6o) active space including valence $\pi$, $n_\text{O}$, $\sigma_\text{CO}$, $\sigma^*_\text{CO}$ and $3p_y$ orbitals. [e]Using reference (4e,4o) active space including valence $\pi$, $\sigma_\text{CO}$ and $\sigma^*_\text{CO}$ orbitals.

Table S13: NEVPT2/aug-cc-pVTZ vertical transition energies (in eV) of acrolein.

| State | Active space $(a', a'')$ | State average $(A', A'')$ | CASSCF | NEVPT2 |
|---|---|---|---|---|
| $^1A''(\mathrm{V}; n \rightarrow \pi^\star)$ | (8,4) | (1,3) | $4.02^a$ | $3.76^a$,$3.73^b$ |
| $^1A'(\mathrm{V}; \pi \rightarrow \pi^\star)$ | (8,4) | (4,0) | $8.24^a$ | $6.67^a$ |
| $^1A''(\mathrm{V}; n \rightarrow \pi^\star)$ | (8,4) | (1,3) | $7.63^a$ | $7.16^{a,c}$,$7.57^{b,c}$ |
| $^1A'(\mathrm{R}; n \rightarrow 3s)$ | (8,4) | (4,0) | $6.98^a$ | $7.05^a$ |
| $^3A''(\mathrm{V}; n \rightarrow \pi^\star)$ | (8,4) | (1,3) | $3.86^a$ | $3.46^a$,$3.44^b$ |
| $^3A'(\mathrm{V}; \pi \rightarrow \pi^\star)$ | (8,4) | (4,0) | $4.31^a$ | $3.95^a$ |
| $^3A'(\mathrm{V}; \pi \rightarrow \pi^\star)$ | (8,4) | (4,0) | $6.76^a$ | $6.23^a$ |
| $^3A''(\mathrm{V}; n \rightarrow \pi^\star)$ | (8,4) | (1,3) | $7.47^a$ | $6.83^{a,d}$,$7.06^{b,d}$ |

[a]Using reference (12e,12o) active space including valence $\pi$, $\sigma_{\mathrm{CC}}$, $\sigma_{\mathrm{CO}}$, $\sigma^*_{\mathrm{CC}}$, $\sigma^*_{\mathrm{CO}}$, $n_{\mathrm{O}}$ and $3s$ orbitals. [b]Using reference (12e,13o) active space including valence $\pi$, $\sigma_{\mathrm{CC}}$, $\sigma_{\mathrm{CO}}$, $\sigma^*_{\mathrm{CC}}$, $\sigma^*_{\mathrm{CO}}$, $n_{\mathrm{O}}$, $3s$ and $3p_z$ orbitals. [c]Substantial Rydberg and doubly-excited character. [d]Substantial doubly-excited character.

Table S14: NEVPT2/aug-cc-pVTZ vertical transition energies (in eV) of benzene.

| State | Active space $(a_g, b_{3u}, b_{2u}, b_{1g}, b_{1u}, b_{2g}, b_{3g}, a_u)$ | State average $(A_g, B_{3u}, B_{2u}, B_{1g}, B_{1u}, B_{2g}, B_{3g}, A_u)$ | CASSCF | NEVPT2 |
|---|---|---|---|---|
| $^1B_{2u}(\mathrm{V}; \pi \rightarrow \pi^\star)$ | (0,0,0,0,2,1,2,1) | (1,1,0,0,0,0,0,0) | $4.98^a$ | $5.32^a$,$5.32^b$ |
| $^1B_{1u}(\mathrm{V}; \pi \rightarrow \pi^\star)$ | (0,0,0,0,4,1,2,2) | (1,1,2,0,0,0,0,0) | $7.27^b$ | $6.01^a$,$6.43^b$ |
| $^1E_{1g}(\mathrm{R}; \pi \rightarrow 3s)$ | (1,0,0,0,2,1,2,1) | (1,0,0,0,0,1,1,0) | $5.90^c$ | $6.75^c$ |
| $^1A_{2u}(\mathrm{R}; \pi \rightarrow 3p)$ | (0,1,1,0,2,1,2,1) | (1,0,0,0,2,0,0,1) | $6.14^d$ | $7.40^d$ |
| $^1E_{2u}(\mathrm{R}; \pi \rightarrow 3p)$ | (0,1,1,0,2,1,2,1) | (1,0,0,0,2,0,0,1) | $6.21^d$ | $7.45^d$ |
| $^3B_{1u}(\mathrm{V}; \pi \rightarrow \pi^\star)$ | (0,0,0,0,4,1,2,2) | (1,0,1,0,0,0,0,0) | $3.85^b$ | $4.44^a$,$4.32^b$ |
| $^3E_{1u}(\mathrm{V}; \pi \rightarrow \pi^\star)$ | (0,0,0,0,4,1,2,2) | (1,1,1,0,0,0,0,0) | $4.85^b$ | $4.99^a$,$4.92^b$ |
| $^3B_{2u}(\mathrm{V}; \pi \rightarrow \pi^\star)$ | (0,0,0,0,4,1,2,2) | (1,1,0,0,0,0,0,0) | $6.75^b$ | $5.30^a$,$5.51^b$ |

[a]Using reference (6e,6o) active space including valence $\pi$ orbitals. [b]Using reference (6e,9o) active space including valence $\pi$ and three $3p_z$ orbitals. [c]Using reference (6e,7o) active space including valence $\pi$ and $3s$ orbitals. [d]Using reference (6e,8o) active space including valence $\pi$, $3p_x$ and $3p_y$ orbitals.

Table S15: NEVPT2/aug-cc-pVTZ vertical transition energies (in eV) of butadiene.

| State | Active space $(a_g, a_u, b_u, b_g)$ | State average $(A_g, A_u, B_u, B_g)$ | CASSCF | NEVPT2 |
|---|---|---|---|---|
| $^1B_u(\mathrm{V}; \pi \to \pi^\star)$ | (0,4,0,4) | (1,0,2,0) | 6.65[c] | 6.04[a],6.73[b],6.68[c] |
| $^1B_g(\mathrm{R}; \pi \to 3s)$ | (4,2,3,2) | (1,0,0,1) | 5.94[d] | 6.44[d] |
| $^1A_g(\mathrm{V}; \pi \to \pi^\star)$ | (3,2,3,2) | (2,0,0,0) | 6.99[a] | 6.70[a] |
| $^1A_u(\mathrm{R}; \pi \to 3p)$ | (3,2,5,2) | (1,2,0,0) | 5.95[e] | 6.84[e] |
| $^1A_u(\mathrm{R}; \pi \to 3p)$ | (3,2,5,2) | (1,2,0,0) | 6.12[e] | 7.01[e] |
| $^1B_u(\mathrm{R}; \pi \to 3p)$ | (0,4,0,4) | (1,0,2,0) | 7.93[c] | 6.99[b],7.45[c] |
| $^3B_u(\mathrm{V}; \pi \to \pi^\star)$ | (3,2,3,2) | (1,0,1,0) | 3.55[a] | 3.40[a] |
| $^3A_g(\mathrm{V}; \pi \to \pi^\star)$ | (3,2,3,2) | (2,0,0,0) | 5.52[a] | 5.30[a] |
| $^3B_g(\mathrm{R}; \pi \to 3s)$ | (4,2,3,2) | (1,0,0,1) | 5.89[d] | 6.38[d] |

[a]Using reference (10e,10o) active space including valence $\pi$, $\sigma_{\mathrm{CC}}$ and $\sigma^*_{\mathrm{CC}}$ orbitals. [b]Using reference (10e,11o) active space including valence $\pi$, $\sigma_{\mathrm{CC}}$, $\sigma^*_{\mathrm{CC}}$ and $3p_z$ orbitals. [c]Using reference (4e,8o) active space including valence $\pi$ and four $3p_z$. [d]Using reference (10e,11o) active space including valence $\pi$, $\sigma_{\mathrm{CC}}$, $\sigma^*_{\mathrm{CC}}$ and $3s$ orbitals. [e]Using reference (10e,12o) active space including valence $\pi$, $\sigma_{\mathrm{CC}}$, $\sigma^*_{\mathrm{CC}}$, $3p_x$ and $3p_y$ orbitals.

Table S16: NEVPT2/aug-cc-pVTZ vertical transition energies (in eV) of cyanoacetylene.

| State | Active space $(a_1, b_1, b_2, a_2)$ | State average $(A_1, B_1, B_2, A_2)$ | CASSCF[a] | NEVPT2[a] |
|---|---|---|---|---|
| $^1\Sigma^-(\mathrm{V}; \pi \to \pi^\star)$ | (0,4,4,0) | (1,0,0,1) | 6.54 | 5.78 |
| $^1\Delta(\mathrm{V}; \pi \to \pi^\star)$ | (0,4,4,0) | (2,0,0,1) | 6.80 | 6.10 |
| $^3\Sigma^+(\mathrm{V}; \pi \to \pi^\star)$ | (0,4,4,0) | (2,0,0,0) | 4.86 | 4.45 |
| $^3\Delta(\mathrm{V}; \pi \to \pi^\star)$ | (0,4,4,0) | (2,0,0,1) | 5.64 | 5.19 |
| $^1A''[\mathrm{F}](\mathrm{V}; \pi \to \pi^\star)$ | ($a'$:4,$a''$:4) | ($A'$:1,$A''$:2) | 4.30 | 3.50 |

[a]All calculations using a full valence $\pi$ active space of (8e,8o).

Table S17: NEVPT2/aug-cc-pVTZ vertical transition energies (in eV) of cyanoformaldehyde.

| State | Active space $(a', a'')$ | State average $(A', A'')$ | CASSCF | NEVPT2 |
|---|---|---|---|---|
| $^1A''(\mathrm{V}; n \to \pi^\star)$ | (3,4) | (1,2) | 4.02[a] | 3.98[a] |
| $^1A''(\mathrm{V}; \pi \to \pi^\star)$ | (3,4) | (1,2) | 7.61[a] | 6.44[a] |
| $^3A''(\mathrm{V}; n \to \pi^\star)$ | (3,4) | (1,1) | 3.52[a] | 3.58[a] |
| $^3A'(\mathrm{V}; \pi \to \pi^\star)$ | (2,4) | (2,0) | 4.98[b] | 5.35[b] |

[a] Using reference (8e,7o) active space including valence $\pi$ and $n_{\mathrm{O}}$ orbitals. [b] Using reference (6e,6o) active space including valence $\pi$ orbitals.

Table S18: NEVPT2/aug-cc-pVTZ vertical transition energies (in eV) of cyanogen.

| State | Active space $(a_g, b_{3u}, b_{2u}, b_{1g}, b_{1u}, b_{2g}, b_{3g}, a_u)$ | State average $(A_g, B_{3u}, B_{2u}, B_{1g}, B_{1u}, B_{2g}, B_{3g}, A_u)$ | CASSCF[a] | NEVPT2[a] |
|---|---|---|---|---|
| $^1\Sigma_u^-(\text{V}; \pi \to \pi^\star)$ | (0,2,2,0,0,2,2,0) | (1,0,0,0,0,0,0,1) | 7.14 | 6.32 |
| $^1\Delta_u(\text{V}; \pi \to \pi^\star)$ | (0,2,2,0,0,2,2,0) | (1,0,0,0,1,0,0,1) | 7.46 | 6.66 |
| $^3\Sigma_u^+(\text{V}; \pi \to \pi^\star)$ | (0,2,2,0,0,2,2,0) | (1,0,0,0,1,0,0,0) | 5.28 | 4.88 |
| $^1\Sigma_u^-[\text{F}](\text{V}; \pi \to \pi^\star)$ | (0,2,2,0,0,2,2,0) | (1,0,0,0,0,0,0,1) | 5.68 | 4.97 |

[a]All calculations using a full valence $\pi$ active space of (8e,8o).

Table S19: NEVPT2/aug-cc-pVTZ vertical transition energies (in eV) of cyclopentadiene.

| State | Active space $(a_1, b_1, b_2, a_2)$ | State average $(A_1, B_1, B_2, A_2)$ | CASSCF | NEVPT2 |
|---|---|---|---|---|
| $^1B_2(\text{V}; \pi \to \pi^\star)$ | (0,4,0,2) | (1,0,2,0) | 6.71[c] | 4.96[a],4.92[b],5.65[c] |
| $^1A_2(\text{R}; \pi \to 3s)$ | (2,2,0,2) | (1,0,0,2) | 5.21[d] | 5.92[d] |
| $^1B_1(\text{R}; \pi \to 3p)$ | (0,2,1,2) | (1,1,0,0) | 6.08[e] | 6.42[e] |
| $^1A_2(\text{R}; \pi \to 3p)$ | (2,2,0,2) | (1,0,0,2) | 5.78[d] | 6.59[d] |
| $^1B_2(\text{R}; \pi \to 3p)$ | (0,4,0,2) | (1,0,2,0) | 6.16[c] | 6.58[b],6.60[c] |
| $^1A_1(\text{V}; \pi \to \pi^\star)$ | (0,2,0,2) | (3,0,0,0) | 6.49[a,f] | 6.75[a,f] |
| $^3B_2(\text{V}; \pi \to \pi^\star)$ | (0,2,0,2) | (1,0,1,0) | 3.26[a] | 3.41[a] |
| $^3A_1(\text{V}; \pi \to \pi^\star)$ | (0,2,0,2) | (3,0,0,0) | 4.92[a] | 5.30[a] |
| $^3A_2(\text{R}; \pi \to 3s)$ | (1,2,0,2) | (1,0,0,1) | 5.53[g] | 5.73[g] |
| $^3B_1(\text{R}; \pi \to 3p)$ | (0,2,1,2) | (1,1,0,0) | 6.05[e] | 6.40[e] |

[a]Using reference (4e,4o) active space including valence $\pi$ orbitals. [b]Using reference (4e,5o) active space including valence $\pi$ and $3p_x$ orbitals. [c]Using reference (4e,6o) active space including valence $\pi$ and two $3p_x$ orbitals. [d]Using reference (4e,6o) active space including valence $\pi$, $3s$ and $3p_z$ orbitals. [e]Using reference (4e,5o) active space including valence $\pi$ and $3p_y$ orbitals. [f]Strong double-excitation character. [g]Using reference (4e,5o) active space including valence $\pi$ and $3s$ orbitals.

Table S20: NEVPT2/aug-cc-pVTZ vertical transition energies (in eV) of cyclopropenone.

| State | Active space $(a_1, b_1, b_2, a_2)$ | State average $(A_1, B_1, B_2, A_2)$ | CASSCF[a] | NEVPT2[a] |
|---|---|---|---|---|
| $^1B_1(\mathrm{V}; n \to \pi^\star)$ | (2,3,1,1) | (1,3,0,0) | 4.92 | 4.04 |
| $^1A_2(\mathrm{V}; n \to \pi^\star)$ | (0,4,2,1) | (1,0,0,3) | 5.64 | 5.85 |
| $^1B_2(\mathrm{R}; n \to 3s)$ | (2,3,1,1) | (1,0,3,0) | 5.68 | 6.51 |
| $^1B_2(\mathrm{V}; \pi \to \pi^\star)$ | (2,3,1,1) | (1,0,3,0) | 6.40 | 6.82 |
| $^1B_2(\mathrm{R}; n \to 3p)$ | (2,3,1,1) | (1,0,3,0) | 6.35 | 7.07 |
| $^1A_1(\mathrm{R}; n \to 3p)$ | (0,4,2,1) | (4,0,0,0) | 6.84 | 7.28 |
| $^1A_1(\mathrm{V}; \pi \to \pi^\star)$ | (0,4,2,1) | (4,0,0,0) | 10.42 | 8.19 |
| $^3B_1(\mathrm{V}; n \to \pi^\star)$ | (2,3,1,1) | (1,3,0,0) | 4.72 | 3.51 |
| $^3B_2(\mathrm{V}; \pi \to \pi^\star)$ | (2,3,1,1) | (1,0,3,0) | 4.39 | 5.10 |
| $^3A_2(\mathrm{V}; n \to \pi^\star)$ | (0,4,2,1) | (1,0,0,3) | 5.40 | 5.60 |
| $^3A_1(\mathrm{V}; \pi \to \pi^\star)$ | (0,4,2,1) | (4,0,0,0) | 6.59 | 7.16 |

[a]All calculations using reference (6e,7o) active space.

Table S21: NEVPT2/aug-cc-pVTZ vertical transition energies (in eV) of cyclopropenethione.

| State | Active space $(a_1, b_1, b_2, a_2)$ | State average $(A_1, B_1, B_2, A_2)$ | CASSCF | NEVPT2 |
|---|---|---|---|---|
| $^1A_2(\mathrm{V}; n \to \pi^\star)$ | (0,3,1,1) | (1,0,0,1) | 3.44[a] | 3.52[a] |
| $^1B_1(\mathrm{V}; n \to \pi^\star)$ | (0,3,1,1) | (1,1,0,0) | 3.57[a] | 3.50[a] |
| $^1B_2(\mathrm{V}; \pi \to \pi^\star)$ | (2,3,1,1) | (1,0,3,0) | 4.51[b] | 4.77[b] |
| $^1B_2(\mathrm{R}; n \to 3s)$ | (2,3,1,1) | (1,0,3,0) | 4.59[b] | 5.35[b] |
| $^1A_1(\mathrm{V}; \pi \to \pi^\star)$ | (0,3,0,1) | (2,0,0,0) | 6.46[c] | 5.54[c] |
| $^1B_2(\mathrm{R}; n \to 3p)$ | (2,3,1,1) | (1,0,3,0) | 5.27[b] | 5.99[b] |
| $^3A_2(\mathrm{V}; n \to \pi^\star)$ | (0,3,1,1) | (1,0,0,1) | 3.26[a] | 3.38[a] |
| $^3B_1(\mathrm{V}; n \to \pi^\star)$ | (0,3,1,1) | (1,1,0,0) | 3.51[a] | 3.40[a] |
| $^3B_2(\mathrm{V}; \pi \to \pi^\star)$ | (2,3,1,1) | (1,0,3,0) | 3.80[b] | 4.21[c],4.17[b] |
| $^3A_1(\mathrm{V}; \pi \to \pi^\star)$ | (0,3,0,1) | (2,0,0,0) | 3.83[c] | 4.13[c] |

[a]Using reference (6e,5o) active space. [b]Using reference (6e,7o) active space. [c]Using reference (4e,4o) active space.

Table S22: NEVPT2/aug-cc-pVTZ vertical transition energies (in eV) of diacetylene.

| State | Active space $(a_g, b_{3u}, b_{2u}, b_{1g}, b_{1u}, b_{2g}, b_{3g}, a_u)$ | State average $(A_g, B_{3u}, B_{2u}, B_{1g}, B_{1u}, B_{2g}, B_{3g}, A_u)$ | CASSCF[a] | NEVPT2[a] |
|---|---|---|---|---|
| $^1\Sigma_u^-(\text{V}; \pi \to \pi^\star)$ | (0,2,2,0,0,2,2,0) | (1,0,0,0,0,0,0,1) | 6.13 | 5.33 |
| $^1\Delta_u(\text{V}; \pi \to \pi^\star)$ | (0,2,2,0,0,2,2,0) | (1,0,0,0,1,0,0,1) | 6.39 | 5.61 |
| $^3\Sigma_u^+(\text{V}; \pi \to \pi^\star)$ | (0,2,2,0,0,2,2,0) | (1,0,0,0,1,0,0,0) | 4.54 | 4.08 |
| $^3\Delta_u(\text{V}; \pi \to \pi^\star)$ | (0,2,2,0,0,2,2,0) | (1,0,0,0,1,0,0,1) | 5.28 | 4.78 |

[a]All calculations using a full valence $\pi$ active space of (8e,8o).

Table S23: NEVPT2/aug-cc-pVTZ vertical transition energies (in eV) of furan.

| State | Active space $(a_1, b_1, b_2, a_2)$ | State average $(A_1, B_1, B_2, A_2)$ | CASSCF | NEVPT2 |
|---|---|---|---|---|
| $^1A_2(\text{R}; \pi \to 3s)$ | (2,3,0,2) | (1,0,0,2) | 5.26[a] | 6.28[a] |
| $^1B_2(\text{V}; \pi \to \pi^\star)$ | (0,4,0,2) | (1,0,2,0) | 7.78[c] | 5.92[b],6.20[c,d] |
| $^1A_1(\text{V}; \pi \to \pi^\star)$ | (0,3,0,2) | (3,0,0,0) | 6.73[b,e] | 6.77[b,e] |
| $^1B_1(\text{R}; \pi \to 3p)$ | (0,3,1,2) | (1,1,0,0) | 6.07[f] | 6.71[f] |
| $^1A_2(\text{R}; \pi \to 3p)$ | (2,3,0,2) | (1,0,0,2) | 5.87[a] | 6.99[a] |
| $^1B_2(\text{R}; \pi \to 3p)$ | (0,4,0,2) | (1,0,2,0) | 6.54[c] | 7.01[c,d] |
| $^3B_2(\text{V}; \pi \to \pi^\star)$ | (0,3,0,2) | (1,0,1,0) | 3.94[b] | 4.42[b] |
| $^3A_1(\text{V}; \pi \to \pi^\star)$ | (0,3,0,2) | (3,0,0,0) | 5.41[b] | 5.60[b] |
| $^3A_2(\text{R}; \pi \to 3s)$ | (1,3,0,2) | (1,0,0,1) | 5.57[g] | 6.08[g] |
| $^3B_1(\text{R}; \pi \to 3p)$ | (0,3,1,2) | (1,1,0,0) | 6.04[f] | 6.68[f] |

[a]Using reference (6e,7o) active space including valence $\pi$, $3s$ and $3p_z$ orbitals. [b]Using reference (6e,5o) active space including valence $\pi$ orbitals. [c]Using reference (6e,6o) active space including valence $\pi$ and $3p_x$ orbitals. [d]Increasing the $\pi$ $3p_x$ active space leads to strong mixing in the zeroth-order wavefunction requiring QD-NEVPT2 (see Pastore et al., Chem. Phys. Lett. 2006, 426, 445–451). [e]Strong double-excitation character. [f]Using reference (6e,6o) active space including valence $\pi$ and $3p_y$ orbitals. [g]Using reference (6e,6o) active space including valence $\pi$ and $3s$ orbitals.

Table S24: NEVPT2/aug-cc-pVTZ vertical transition energies (in eV) of glyoxal.

| State | Active space $(a_g, a_u, b_u, b_g)$ | State average $(A_g, A_u, B_u, B_g)$ | CASSCF | NEVPT2 |
|---|---|---|---|---|
| $^1A_u(\text{V}; n \to \pi^\star)$ | (4,2,4,2) | (1,1,0,0) | $3.42^a$ | $2.90^a$ |
| $^1B_g(\text{V}; n \to \pi^\star)$ | (4,2,4,3) | (1,0,0,2) | $4.68^b$ | $4.31^a$,$4.30^b$ |
| $^1A_g(\text{V}; n, n \to \pi^\star, \pi^\star)$ | (4,2,4,2) | (2,0,0,0) | $5.92^a$ | $5.52^a$ |
| $^1B_g(\text{V}; n \to \pi^\star)$ | (4,2,4,3) | (1,0,0,2) | $7.35^b$ | $6.91^{a,c}$,$6.64^{b,c}$ |
| $^1B_u(\text{R}; n \to 3p)$ | (4,2,5,2) | (1,0,1,0) | $7.04^d$ | $7.84^d$ |
| $^3A_u(\text{V}; n \to \pi^\star)$ | (4,2,4,2) | (1,1,0,0) | $3.06^a$ | $2.49^a$ |
| $^3B_g(\text{V}; n \to \pi^\star)$ | (4,2,4,2) | (1,0,0,1) | $4.61^a$ | $3.99^a$ |
| $^3B_u(\text{V}; \pi \to \pi^\star)$ | (4,2,4,2) | (1,0,1,0) | $5.46^a$ | $5.17^a$ |
| $^3A_g(\text{V}; \pi \to \pi^\star)$ | (4,2,4,2) | (2,0,0,0) | $6.69^a$ | $6.33^a$ |

[a]Using reference (14e,12o) active space including valence $\pi$, two $n_\text{O}$, $\sigma_\text{CC}$, $\sigma_\text{CO}$, $\sigma^*_\text{CC}$ and $\sigma^*_\text{CO}$ orbitals. [b]Using reference (14e,13o) active space including valence $\pi$, two $n_\text{O}$, $\sigma_\text{CC}$, $\sigma_\text{CO}$, $\sigma^*_\text{CC}$, $\sigma^*_\text{CO}$ and $3p_z$ orbitals. [c]Non-negligible doubly-excited and Rydberg character. [d]Using reference (14e,13o) active space including valence $\pi$, two $n_\text{O}$, $\sigma_\text{CC}$, $\sigma_\text{CO}$, $\sigma^*_\text{CC}$, $\sigma^*_\text{CO}$ and $3p_x$ orbitals.

Table S25: NEVPT2/aug-cc-pVTZ vertical transition energies (in eV) of imidazole.

| State | Active space $(a', a'')$ | State average $(A', A'')$ | CASSCF | NEVPT2 |
|---|---|---|---|---|
| $^1A''(\text{R}; \pi \to 3s)$ | (2,5) | (1,3) | $5.04^b$ | $5.97^a$,$5.93^b$ |
| $^1A'(\text{V}; \pi \to \pi^\star)$ | (0,9) | (3,0) | $6.18^e$ | $6.86^c$,$6.81^d$,$6.73^e$ |
| $^1A''(\text{V}; n \to \pi^\star)$ | (2,5) | (1,3) | $7.13^b$ | $6.97^f$,$6.96^b$ |
| $^1A'(\text{R}; \pi \to 3p)$ | (0,9) | (3,0) | $6.73^e$ | $7.08^d$,$7.00^e$ |
| $^3A'(\text{V}; \pi \to \pi^\star)$ | (0,9) | (3,0) | $4.55^e$ | $4.98^c$,$4.86^e$ |
| $^3A''(\text{R}; \pi \to 3s)$ | (2,5) | (1,3) | $5.03^b$ | $5.93^a$,$5.91^b$ |
| $^3A'(\text{V}; \pi \to \pi^\star)$ | (0,9) | (3,0) | $5.69^e$ | $6.09^c$,$5.91^e$ |
| $^3A''(\text{V}; n \to \pi^\star)$ | (2,5) | (1,3) | $6.58^b$ | $6.49^f$,$6.48^b$ |

[a]Using reference (6e,6o) active space including valence $\pi$ and $3s$ orbitals. [b]Using reference (8e,7o) active space including valence $\pi$, $n_\text{N}$ and $3s$ orbitals. [c]Using reference (6e,5o) active space including valence $\pi$ orbitals. [d]Using reference (6e,6o) active space including valence $\pi$ and one $3p_z$ orbitals. [e]Using reference (6e,9o) active space including valence $\pi$ and four $3p_z$ orbitals. [f]Using reference (8e,6o) active space including valence $\pi$ and $n_\text{N}$ orbitals.

Table S26: NEVPT2/aug-cc-pVTZ vertical transition energies (in eV) of isobutene.

| State | Active space $(a_1, b_1, b_2, a_2)$ | State average $(A_1, B_1, B_2, A_2)$ | CASSCF | NEVPT2 |
|---|---|---|---|---|
| $^1B_1(\mathrm{R}; \pi \rightarrow 3s)$ | (3,2,0,0) | (1,1,0,0) | 6.12$^a$ | 6.63$^a$ |
| $^1A_1(\mathrm{R}; \pi \rightarrow 3p)$ | (2,3,0,0) | (2,0,0,0) | 6.90$^b$ | 7.20$^b$ |
| $^3A_1(\mathrm{V}; \pi \rightarrow \pi^\star)$ | (2,2,0,0) | (2,0,0,0) | 4.66$^c$ | 4.61$^c$ |

$^a$Using reference (4e,5o) active space including valence $\pi$, $\sigma_{\mathrm{CC}}$, $\sigma^*_{\mathrm{CC}}$ and $3s$ orbitals. $^b$Using reference (4e,5o) active space including valence $\pi$, $\sigma_{\mathrm{CC}}$, $\sigma^*_{\mathrm{CC}}$ and $3p_x$ orbitals. $^c$Using reference (4e,4o) active space including valence $\pi$, $\sigma_{\mathrm{CC}}$ and $\sigma^*_{\mathrm{CC}}$ orbitals.

Table S27: NEVPT2/aug-cc-pVTZ vertical transition energies (in eV) of methylenecyclopropene.

| State | Active space $(a_1, b_1, b_2, a_2)$ | State average $(A_1, B_1, B_2, A_2)$ | CASSCF | NEVPT2 |
|---|---|---|---|---|
| $^1B_2(\mathrm{V}; \pi \rightarrow \pi^\star)$ | (0,3,0,1) | (1,0,1,0) | 4.47$^a$ | 4.37$^a$ |
| $^1B_1(\mathrm{R}; \pi \rightarrow 3s)$ | (1,3,0,1) | (1,1,0,0) | 4.92$^c$ | 5.51$^b$,5.49$^c$ |
| $^1A_2(\mathrm{R}; \pi \rightarrow 3p)$ | (0,3,1,1) | (1,0,0,1) | 5.37$^c$ | 6.00$^c$ |
| $^1A_1(\mathrm{V}; \pi \rightarrow \pi^\star)$ | (0,6,0,1) | (5,0,0,0) | 5.37$^e$ | 6.33$^d$,6.36$^e$ |
| $^3B_2(\mathrm{V}; \pi \rightarrow \pi^\star)$ | (0,3,0,1) | (1,0,1,0) | 3.44$^a$ | 3.66$^a$ |
| $^3A_1(\mathrm{V}; \pi \rightarrow \pi^\star)$ | (0,5,0,1) | (4,0,0,0) | 4.60$^d$ | 4.87$^d$ |

$^a$Using reference (4e,4o) active space. $^b$Using reference (6e,6o) active space. $^c$Using reference (4e,5o) active space. $^d$Using reference (4e,6o) active space. $^e$Using reference (4e,7o) active space.

Table S28: NEVPT2/aug-cc-pVTZ vertical transition energies (in eV) of propynal.

| State | Active space $(a', a'')$ | State average $(A', A'')$ | CASSCF | NEVPT2 |
|---|---|---|---|---|
| $^1A''(\mathrm{V}; n \rightarrow \pi^\star)$ | (3,4) | (1,2) | 4.00$^a$ | 3.95$^a$ |
| $^1A''(\mathrm{V}; \pi \rightarrow \pi^\star)$ | (3,4) | (1,2) | 6.62$^a$ | 5.50$^a$ |
| $^3A''(\mathrm{V}; n \rightarrow \pi^\star)$ | (3,4) | (1,1) | 3.52$^a$ | 3.59$^a$ |
| $^3A'(\mathrm{V}; \pi \rightarrow \pi^\star)$ | (2,4) | (2,0) | 4.69$^b$ | 4.63$^b$ |

$^a$Using reference (8e,7o) active space including valence $\pi$ and $n_{\mathrm{O}}$ orbitals. $^b$Using reference (6e,6o) active space including valence $\pi$ orbitals.

Table S29: NEVPT2/aug-cc-pVTZ vertical transition energies (in eV) of pyrazine.

| State | Active space $(a_g, b_{3u}, b_{2u}, b_{1g}, b_{1u}, b_{2g}, b_{3g}, a_u)$ | State average $(A_g, B_{3u}, B_{2u}, B_{1g}, B_{1u}, B_{2g}, B_{3g}, A_u)$ | CASSCF | NEVPT2 |
|---|---|---|---|---|
| $^1B_{3u}(\mathrm{V}; n \rightarrow \pi^\star)$ | (1,2,0,1,1,2,0,1) | (1,1,0,0,0,0,0,0) | 4.76[a] | 4.17[a] |
| $^1A_{u}(\mathrm{V}; n \rightarrow \pi^\star)$ | (1,2,0,1,1,2,0,1) | (1,0,0,0,0,0,0,1) | 5.90[a] | 4.77[a] |
| $^1B_{2u}(\mathrm{V}; \pi \rightarrow \pi^\star)$ | (0,2,0,1,0,2,0,1) | (1,0,1,0,0,0,0,0) | 4.97[b] | 5.32[b],5.37[c] |
| $^1B_{2g}(\mathrm{V}; n \rightarrow \pi^\star)$ | (1,2,0,1,1,2,0,1) | (1,0,0,0,0,1,0,0) | 5.80[a] | 5.88[a] |
| $^1A_{g}(\mathrm{R}; n \rightarrow 3s)$ | (2,2,0,1,1,2,0,1) | (2,0,0,0,0,0,0,0) | 6.69[d] | 6.70[d] |
| $^1B_{1g}(\mathrm{V}; n \rightarrow \pi^\star)$ | (1,2,0,1,1,2,0,1) | (1,0,0,1,0,0,0,0) | 7.16[a] | 6.75[a] |
| $^1B_{1u}(\mathrm{V}; \pi \rightarrow \pi^\star)$ | (0,4,0,1,0,2,0,2) | (1,0,0,0,3,0,0,0) | 8.04[f] | 6.38[b],6.31[e],6.81[f] |
| $^1B_{1g}(\mathrm{R}; \pi \rightarrow 3s)$ | (1,2,0,1,0,2,0,1) | (1,0,0,1,0,0,0,0) | 6.73[g] | 7.33[g] |
| $^1B_{2u}(\mathrm{R}; n \rightarrow 3p)$ | (1,2,1,1,1,2,0,1) | (1,0,2,0,0,0,0,0) | 7.49[c] | 7.25[c] |
| $^1B_{1u}(\mathrm{R}; n \rightarrow 3p)$ | (1,2,0,1,2,2,0,1) | (1,0,0,0,3,0,0,0) | 7.83[e] | 7.42[e] |
| $^1B_{1u}(\mathrm{V}; \pi \rightarrow \pi^\star)$ | (0,4,0,1,0,2,0,2) | (1,0,0,0,3,0,0,0) | 9.65[f] | 7.29[b],6.96[e],8.25[f] |
| $^3B_{3u}(\mathrm{V}; n \rightarrow \pi^\star)$ | (1,2,0,1,1,2,0,1) | (1,1,0,0,0,0,0,0) | 4.16[a] | 3.56[a] |
| $^3B_{1u}(\mathrm{V}; \pi \rightarrow \pi^\star)$ | (0,4,0,1,0,2,0,2) | (1,0,0,0,2,0,0,0) | 3.98[f] | 4.68[b],4.57[f] |
| $^3B_{2u}(\mathrm{V}; \pi \rightarrow \pi^\star)$ | (0,2,0,1,0,2,0,1) | (1,0,1,0,0,0,0,0) | 4.62[b] | 4.42[b] |
| $^3A_{u}(\mathrm{V}; n \rightarrow \pi^\star)$ | (1,2,0,1,1,2,0,1) | (1,0,0,0,0,0,0,1) | 5.85[a] | 4.75[a] |
| $^3B_{2g}(\mathrm{V}; n \rightarrow \pi^\star)$ | (1,2,0,1,1,2,0,1) | (1,0,0,0,0,1,0,0) | 5.25[a] | 5.21[a] |
| $^3B_{1u}(\mathrm{V}; \pi \rightarrow \pi^\star)$ | (0,4,0,1,0,2,0,2) | (1,0,0,0,2,0,0,0) | 5.15[f] | 5.43[b],5.35[f] |

[a]Using reference (10e,8o) active space including valence $\pi$ and $n_\mathrm{N}$ orbitals. [b]Using reference (6e,6o) active space including valence $\pi$ orbitals. [c]Using reference (10e,9o) active space including valence $\pi$, $n_\mathrm{N}$ and $3p_y$ orbitals. [d]Using reference (10e,9o) active space including valence $\pi$, $n_\mathrm{N}$ and $3s$ orbitals. [e]Using reference (10e,9o) active space including valence $\pi$, $n_\mathrm{N}$ and $3p_z$ orbitals. [f]Using reference (6e,9o) active space including valence $\pi$ and three $3p_x$ orbitals. [g]Using reference (6e,7o) active space including valence $\pi$ and $3s$ orbitals.

Table S30: NEVPT2/aug-cc-pVTZ vertical transition energies (in eV) of pyridazine.

| State | Active space $(a_1, b_1, b_2, a_2)$ | State average $(A_1, B_1, B_2, A_2)$ | CASSCF | NEVPT2 |
|---|---|---|---|---|
| $^1B_1(\text{V}; n \rightarrow \pi^\star)$ | (1,3,1,3) | (1,1,0,0) | 4.29[a] | 3.80[a] |
| $^1A_2(\text{V}; n \rightarrow \pi^\star)$ | (1,3,1,3) | (1,0,0,1) | 4.83[a] | 4.40[a] |
| $^1A_1(\text{V}; \pi \rightarrow \pi^\star)$ | (0,3,0,3) | (2,0,0,0) | 5.12[b] | 5.58[b] |
| $^1A_2(\text{V}; n \rightarrow \pi^\star)$ | (1,3,1,3) | (1,0,0,2) | 6.26[a] | 5.88[a] |
| $^1B_2(\text{R}; n \rightarrow 3s)$ | (2,3,1,3) | (1,0,1,0) | 5.99[c] | 6.21[c] |
| $^1B_1(\text{V}; n \rightarrow \pi^\star)$ | (1,3,1,3) | (1,2,0,0) | 7.16[a] | 6.64[a] |
| $^1B_2(\text{V}; \pi \rightarrow \pi^\star)$ | (0,6,0,6) | (1,0,3,0) | 7.58[e] | 7.82[b],7.19[d],7.10[e] |
| $^3B_1(\text{V}; n \rightarrow \pi^\star)$ | (1,3,1,3) | (1,1,0,0) | 3.60[a] | 3.13[a] |
| $^3A_2(\text{V}; n \rightarrow \pi^\star)$ | (1,3,1,3) | (1,0,0,1) | 4.49[a] | 4.14[a] |
| $^3B_2(\text{V}; \pi \rightarrow \pi^\star)$ | (0,6,0,6) | (1,0,1,0) | 4.06[e] | 4.65[b],4.55[d],4.49[e] |
| $^3A_1(\text{V}; \pi \rightarrow \pi^\star)$ | (0,3,0,3) | (2,0,0,0) | 4.93[b] | 4.94[b] |

[a]Using reference (10e,8o) active space including valence $\pi$ and $n_\text{N}$ orbitals. [b]Using reference (6e,6o) active space including valence $\pi$ orbitals. [c]Using reference (10e,9o) active space including valence $\pi$, $n_\text{N}$ and $3s$ orbitals. [d]Using reference (6e,9o) active space including valence $\pi$, $n_\text{N}$ and three $3p_x$ orbitals. [e]Using reference (6e,12o) active space including valence $\pi$, $n_\text{N}$ and six $3p_x$ orbitals.

Table S31: NEVPT2/aug-cc-pVTZ vertical transition energies (in eV) of pyridine.

| State | Active space $(a_1, b_1, b_2, a_2)$ | State average $(A_1, B_1, B_2, A_2)$ | CASSCF | NEVPT2 |
|---|---|---|---|---|
| $^1B_1(\mathrm{V}; n \to \pi^\star)$ | (1,4,1,2) | (1,2,0,0) | 5.43$^b$ | 5.17$^a$,5.15$^b$ |
| $^1B_2(\mathrm{V}; \pi \to \pi^\star)$ | (0,7,0,3) | (1,0,2,0) | 5.03$^d$ | 5.44$^c$,5.31$^d$ |
| $^1A_2(\mathrm{V}; n \to \pi^\star)$ | (2,4,0,2) | (1,0,0,2) | 6.30$^e$ | 5.32$^a$,5.29$^e$ |
| $^1A_1(\mathrm{V}; \pi \to \pi^\star)$ | (0,4,0,2) | (2,0,0,0) | 7.90$^c$ | 6.69$^c$ |
| $^1A_1(\mathrm{R}; n \to 3s)$ | (2,4,0,2) | (2,0,0,0) | 6.40$^e$ | 6.99$^e$ |
| $^1A_2(\mathrm{R}; \pi \to 3s)$ | (2,4,0,2) | (1,0,0,2) | 6.60$^e$ | 6.96$^f$,6.86$^e$ |
| $^1B_2(\mathrm{V}; \pi \to \pi^\star)$ | (0,7,0,3) | (1,0,2,0) | 7.45$^d$ | 8.61$^a$,7.83$^d$ |
| $^1B_1(\mathrm{R}; \pi \to 3p)$ | (1,4,1,2) | (1,2,0,0) | 7.12$^b$ | 7.57$^g$,7.45$^b$ |
| $^1A_1(\mathrm{V}; \pi \to \pi^\star)$ | (0,4,0,2) | (4,0,0,0) | 9.49$^c$ | 6.97$^c$ |
| $^3A_1(\mathrm{V}; \pi \to \pi^\star)$ | (0,4,0,2) | (2,0,0,0) | 3.98$^c$ | 4.60$^c$ |
| $^3B_1(\mathrm{V}; n \to \pi^\star)$ | (1,4,0,2) | (1,1,0,0) | 4.65$^a$ | 4.58$^a$ |
| $^3B_2(\mathrm{V}; \pi \to \pi^\star)$ | (0,7,0,3) | (1,0,2,0) | 4.83$^d$ | 4.90$^c$,4.88$^d$ |
| $^3A_1(\mathrm{V}; \pi \to \pi^\star)$ | (0,4,0,2) | (3,0,0,0) | 5.11$^c$ | 5.19$^c$ |
| $^3A_2(\mathrm{V}; n \to \pi^\star)$ | (1,4,0,2) | (1,0,0,1) | 5.94$^a$ | 5.33$^a$ |
| $^3B_2(\mathrm{V}; \pi \to \pi^\star)$ | (0,7,0,3) | (1,0,2,0) | 6.93$^d$ | 7.00$^c$,6.29$^d$ |

$^a$Using reference (8e,7o) active space including valence $\pi$ and $n_\mathrm{N}$ orbitals. $^b$Using reference (8e,8o) active space including valence $\pi$, $n_\mathrm{N}$ and $3p_y$ orbitals. $^c$Using reference (6e,6o) active space including valence $\pi$ orbitals. $^d$Using reference (6e,10o) active space including valence $\pi$ and four $3p_x$ orbitals. $^e$Using reference (8e,8o) active space including valence $\pi$, $n_\mathrm{N}$ and $3s$ orbitals. $^d$Using reference (6e,8o) active space including valence $\pi$ and $3s$ orbitals. $^g$Using reference (6e,7o) active space including valence $\pi$ and $3p_y$ orbitals.

Table S32: NEVPT2/aug-cc-pVTZ vertical transition energies (in eV) of pyrimidine.

| State | Active space $(a_1, b_1, b_2, a_2)$ | State average $(A_1, B_1, B_2, A_2)$ | CASSCF | NEVPT2 |
|---|---|---|---|---|
| $^1B_1(\text{V}; n \rightarrow \pi^\star)$ | (1,4,1,2) | (1,1,0,0) | $4.85^a$ | $4.55^a$ |
| $^1A_2(\text{V}; n \rightarrow \pi^\star)$ | (1,4,1,2) | (1,0,0,1) | $5.52^a$ | $4.84^a$ |
| $^1B_2(\text{V}; \pi \rightarrow \pi^\star)$ | (0,7,0,4) | (1,0,1,0) | $5.23^e$ | $5.71^b$,$5.57^d$,$5.53^e$ |
| $^1A_2(\text{V}; n \rightarrow \pi^\star)$ | (1,4,1,2) | (1,0,0,2) | $6.70^a$ | $6.02^a$ |
| $^1B_1(\text{V}; n \rightarrow \pi^\star)$ | (1,4,1,2) | (1,2,0,0) | $7.20^a$ | $6.40^a$ |
| $^1B_2(\text{R}; n \rightarrow 3s)$ | (2,4,1,2) | (1,0,2,0) | $6.86^c$ | $6.77^c$ |
| $^1A_1(\text{V}; \pi \rightarrow \pi^\star)$ | (0,7,0,4) | (2,0,0,0) | $7.62^e$ | $7.47^b$,$7.11^e$ |
| $^3B_1(\text{V}; n \rightarrow \pi^\star)$ | (1,4,1,2) | (1,1,0,0) | $4.45^a$ | $4.17^a$ |
| $^3A_1(\text{V}; \pi \rightarrow \pi^\star)$ | (0,7,0,4) | (2,0,0,0) | $4.25^e$ | $4.84^b$,$4.67^e$ |
| $^3A_2(\text{V}; n \rightarrow \pi^\star)$ | (1,4,1,2) | (1,0,0,1) | $5.20^a$ | $4.72^a$ |
| $^3B_2(\text{V}; \pi \rightarrow \pi^\star)$ | (0,7,0,4) | (1,0,1,0) | $5.00^e$ | $5.08^b$,$5.01^e$ |

[a]Using reference (10e,8o) active space including valence $\pi$ and $n_\text{N}$ orbitals [b]Using reference (6e,6o) active space including valence $\pi$ orbitals. [c]Using reference (10e,9o) active space including valence $\pi$, $n_\text{N}$ and $3s$ orbitals. [d]Using reference (6e,9o) active space including valence $\pi$ and three $3p_x$ orbitals. [e]Using reference (6e,11o) active space including valence $\pi$ and five $3p_x$ orbitals.

Table S33: NEVPT2/aug-cc-pVTZ vertical transition energies (in eV) of pyrrole.

| State | Active space $(a_1, b_1, b_2, a_2)$ | State average $(A_1, B_1, B_2, A_2)$ | CASSCF | NEVPT2 |
|---|---|---|---|---|
| $^1A_2(\text{R}; \pi \rightarrow 3s)$ | (1,3,0,2) | (1,0,0,1) | $4.49^a$ | $5.51^a$ |
| $^1B_1(\text{R}; \pi \rightarrow 3p)$ | (0,3,1,2) | (1,1,0,0) | $5.22^b$ | $6.32^b$ |
| $^1A_2(\text{R}; \pi \rightarrow 3p)$ | (2,3,0,2) | (1,0,0,2) | $4.89^c$ | $6.44^c$ |
| $^1B_2(\text{V}; (\pi \rightarrow \pi^\star)$ | (0,4,0,2) | (1,0,2,0) | $7.73^e$ | $6.48^{e,f}$ |
| $^1A_1(\text{V}; \pi \rightarrow \pi^\star)$ | (0,3,0,2) | (3,0,0,0) | $6.47^d$ | $6.53^d$ |
| $^1B_2(\text{R}; \pi \rightarrow 3p)$ | (0,4,0,2) | (1,0,2,0) | $5.82^e$ | $6.50^d$,$6.62^{e,f}$ |
| $^3B_2(\text{V}; \pi \rightarrow \pi^\star)$ | (0,3,0,2) | (1,0,1,0) | $4.24^d$ | $4.74^d$ |
| $^3A_2(\text{R}; \pi \rightarrow 3s)$ | (1,3,0,2) | (1,0,0,1) | $4.47^a$ | $5.49^a$ |
| $^3A_1(\text{V}; \pi \rightarrow \pi^\star)$ | (0,3,0,2) | (3,0,0,0) | $5.52^d$ | $5.56^d$ |
| $^3B_1(\text{R}; \pi \rightarrow 3p)$ | (0,3,1,2) | (1,1,0,0) | $5.18^b$ | $6.28^b$ |

[a]Using reference (6e,6o) active space including valence $\pi$ and $3s$ orbitals. [b]Using reference (6e,6o) active space including valence $\pi$ and $3p_y$ orbitals. [c]Using reference (6e,7o) active space including valence $\pi$, $3s$ and $3p_z$ orbitals. [d]Using reference (6e,5o) active space including valence $\pi$ orbitals. [e]Using reference (6e,6o) active space including valence $\pi$ and $3p_x$ orbitals. [f]Increasing the $\pi$ $3p_x$ active space leads to strong mixing in the zeroth-order wavefunction requiring a multi-state treatment (see Roos et al., J. Chem. Phys. 2002, 116, 7526–7536).

Table S34: NEVPT2/aug-cc-pVTZ vertical transition energies (in eV) of tetrazine.

| State | Active space $(a_g, b_{3u}, b_{2u}, b_{1g}, b_{1u}, b_{2g}, b_{3g}, a_u)$ | State average $(A_g, B_{3u}, B_{2u}, B_{1g}, B_{1u}, B_{2g}, B_{3g}, A_u)$ | CASSCF | NEVPT2 |
|---|---|---|---|---|
| $^1B_{3u}(\text{V}; n \to \pi^\star)$ | (1,2,1,1,1,2,1,1) | (1,1,0,0,0,0,0,0) | $2.99^a$ | $2.35^a$ |
| $^1A_u(\text{V}; n \to \pi^\star)$ | (1,2,1,1,1,2,1,1) | (1,0,0,0,0,0,0,1) | $4.37^a$ | $3.58^a$ |
| $^1A_g(\text{V}; n, n \to \pi^\star, \pi^\star)$ | (1,2,1,1,1,2,1,1) | (2,0,0,0,0,0,0,0) | $5.42^a$ | $4.61^a$ |
| $^1B_{1g}(\text{V}; n \to \pi^\star)$ | (1,2,1,1,1,2,1,1) | (1,0,0,1,0,0,0,0) | $5.41^a$ | $4.95^a$ |
| $^1B_{2u}(\text{V}; \pi \to \pi^\star)$ | (0,2,0,1,0,2,0,1) | (1,0,1,0,0,0,0,0) | $5.04^b$ | $5.56^b$ |
| $^1B_{2g}(\text{V}; n \to \pi^\star)$ | (1,2,1,1,1,2,1,1) | (1,0,0,0,0,1,0,0) | $5.43^a$ | $5.63^a$ |
| $^1A_u(\text{V}; n \to \pi^\star)$ | (1,2,1,1,1,2,1,1) | (1,0,0,0,0,0,0,2) | $6.37^a$ | $5.62^a$ |
| $^1B_{3g}(\text{V}; n, n \to \pi^\star, \pi^\star)$ | (1,2,1,1,1,2,1,1) | (1,0,0,0,0,0,1,0) | $6.59^a$ | $6.15^a$ |
| $^1B_{2g}(\text{V}; n \to \pi^\star)$ | (1,2,1,1,1,2,1,1) | (1,0,0,0,0,2,0,0) | $6.79^a$ | $6.13^a$ |
| $^1B_{1g}(\text{V}; n \to \pi^\star)$ | (1,2,1,1,1,2,1,1) | (1,0,0,2,0,0,0,0) | $7.18^a$ | $6.76^a$ |
| $^3B_{3u}(\text{V}; n \to \pi^\star)$ | (1,2,1,1,1,2,1,1) | (1,1,0,0,0,0,0,0) | $2.38^a$ | $1.73^a$ |
| $^3A_u(\text{V}; n \to \pi^\star)$ | (1,2,1,1,1,2,1,1) | (1,0,0,0,0,0,0,1) | $4.06^a$ | $3.36^a$ |
| $^3B_{1g}(\text{V}; n \to \pi^\star)$ | (1,2,1,1,1,2,1,1) | (1,0,0,1,0,0,0,0) | $4.66^a$ | $4.24^a$ |
| $^3B_{1u}(\text{V}; \pi \to \pi^\star)$ | (0,4,0,1,0,2,0,2) | (1,0,0,0,2,0,0,0) | $3.90^c$ | $4.80^b$,$4.70^a$ |
| $^3B_{2u}(\text{V}; \pi \to \pi^\star)$ | (0,2,0,1,0,2,0,1) | (1,0,1,0,0,0,0,0) | $4.68^b$ | $4.58^b$ |
| $^3B_{2g}(\text{V}; n \to \pi^\star)$ | (1,2,1,1,1,2,1,1) | (1,0,0,0,0,1,0,0) | $5.17^a$ | $5.27^a$ |
| $^3A_u(\text{V}; n \to \pi^\star)$ | (1,2,1,1,1,2,1,1) | (1,0,0,0,0,0,0,2) | $6.12^a$ | $5.13^a$ |
| $^3B_{3g}(\text{V}; n, n \to \pi^\star, \pi^\star)$ | (1,2,1,1,1,2,1,1) | (1,0,0,0,0,0,1,0) | $6.56^a$ | $5.51^a$ |
| $^3B_{1u}(\text{V}; \pi \to \pi^\star)$ | (0,4,0,1,0,2,0,2) | (1,0,0,0,2,0,0,0) | $5.32^c$ | $5.64^b$,$5.56^c$ |

[a]Using reference (14e,10o) active space including valence $\pi$ and $n_\text{N}$ orbitals. [b]Using reference (6e,6o) active space including valence $\pi$ orbitals. [c]Using reference (6e,9o) active space including valence $\pi$ and three $3p_x$ orbitals.

Table S35: NEVPT2/aug-cc-pVTZ vertical transition energies (in eV) of thioacetone.

| State | Active space $(a_1, b_1, b_2, a_2)$ | State average $(A_1, B_1, B_2, A_2)$ | CASSCF | NEVPT2 |
|---|---|---|---|---|
| $^1A_2(\text{V}; n \to \pi^\star)$ | (2,2,1,0) | (1,0,0,1) | $2.72^a$ | $2.55^a$ |
| $^1B_2(\text{R}; n \to 4s)$ | (4,2,1,0) | (1,0,2,0) | $4.80^b$ | $5.72^b$ |
| $^1A_1(\text{V}; \pi \to \pi^\star)$ | (2,2,2,0) | (3,0,0,0) | $6.94^d$ | $6.09^c$,$6.24^d$ |
| $^1B_2(\text{R}; n \to 4p)$ | (4,2,1,0) | (1,0,2,0) | $5.57^b$ | $6.62^b$ |
| $^1A_1(\text{R}; n \to 4p)$ | (2,2,2,0) | (3,0,0,0) | $6.24^d$ | $6.52^d$ |
| $^3A_2(\text{V}; n \to \pi^\star)$ | (2,2,1,0) | (1,0,0,1) | $2.52^a$ | $2.32^a$ |
| $^3A_1(\text{V}; \pi \to \pi^\star)$ | (2,2,0,0) | (2,0,0,0) | $3.52^c$ | $3.48^c$ |

[a]Using reference (6e,5o) active space including valence $\pi$, $n_\text{O}$, $\sigma_\text{CO}$ and $\sigma^*_\text{CO}$ orbitals. [b]Using reference (6e,7o) active space including valence $\pi$, $n_\text{O}$, $\sigma_\text{CO}$, $\sigma^*_\text{CO}$, 4s and $4p_z$ orbitals. [c]Using reference (4e,4o) active space including valence $\pi$, $\sigma_\text{CO}$ and $\sigma^*_\text{CO}$ orbitals. [d]Using reference (6e,6o) active space including valence $\pi$, $n_\text{O}$, $\sigma_\text{CO}$, $\sigma^*_\text{CO}$ and $4p_y$ orbitals.

Table S36: NEVPT2/aug-cc-pVTZ vertical transition energies (in eV) of thiophene.

| State | Active space $(a_1, b_1, b_2, a_2)$ | State average $(A_1, B_1, B_2, A_2)$ | CASSCF | NEVPT2 |
|---|---|---|---|---|
| $^1A_1(\mathrm{V}; \pi \rightarrow \pi^\star)$ | (0,3,0,2) | (3,0,0,0) | $6.11^a$ | $5.84^a$ |
| $^1B_2(\mathrm{V}; \pi \rightarrow \pi^\star)$ | (0,5,0,2) | (1,0,2,0) | $6.94^c$ | $5.64^a$,$5.54^b$,$6.10^c$ |
| $^1A_2(\mathrm{R}; \pi \rightarrow 3s)$ | (1,3,0,2) | (1,0,0,1) | $5.70^d$ | $6.20^d$ |
| $^1B_1(\mathrm{R}; \pi \rightarrow 3p)$ | (0,3,1,2) | (1,1,0,0) | $6.02^e$ | $6.19^e$ |
| $^1A_2(\mathrm{R}; \pi \rightarrow 3p)$ | (0,3,1,2) | (1,0,0,1) | $6.05^e$ | $6.40^e$,$6.52^f$ |
| $^1B_1(\mathrm{R}; \pi \rightarrow 3s)$ | (1,3,1,2) | (1,2,0,0) | $5.78^f$ | $6.73^d$, $6.71^f$ |
| $^1B_2(\mathrm{R}; \pi \rightarrow 3p)$ | (0,5,0,2) | (1,0,2,0) | $6.80^c$ | $7.42^b$,$7.25^c$ |
| $^1A_1(\mathrm{V}; \pi \rightarrow \pi^\star)$ | (0,3,0,2) | (3,0,0,0) | $8.29^{a,g}$ | $7.39^{a,g}$ |
| $^3B_2(\mathrm{V}; \pi \rightarrow \pi^\star)$ | (0,3,0,2) | (1,0,1,0) | $3.68^a$ | $4.13^a$ |
| $^3A_1(\mathrm{V}; \pi \rightarrow \pi^\star)$ | (0,3,0,2) | (3,0,0,0) | $4.97^a$ | $4.84^a$ |
| $^3B_1(\mathrm{R}; \pi \rightarrow 3p)$ | (0,3,1,2) | (1,1,0,0) | $5.86^e$ | $5.98^e$ |
| $^3A_2(\mathrm{R}; \pi \rightarrow 3s)$ | (1,3,0,2) | (1,0,0,1) | $5.65^d$ | $6.14^d$ |

[a]Using reference (6e,5o) active space including valence $\pi$ orbitals. [b]Using reference (6e,6o) active space including valence $\pi$ and $3p_x$ orbitals. [c]Using reference (6e,7o) active space including valence $\pi$ and two $3p_x$ orbitals. [d]Using reference (6e,6o) active space including valence $\pi$ and $3s$ orbitals. [e]Using reference (6e,6o) active space including valence $\pi$ and $3p_y$ orbitals. [f]Using reference (6e,7o) active space including valence $\pi$, $3s$ and $3p_y$ orbitals. [g]Strong double-excitation character.

Table S37: NEVPT2/aug-cc-pVTZ vertical transition energies (in eV) of thiopropynal.

| State | Active space $(a', a'')$ | State average $(A', A'')$ | CASSCF[a] | NEVPT2[a] |
|---|---|---|---|---|
| $^1A''(\mathrm{V}; n \rightarrow \pi^\star)$ | (3,4) | (1,1) | 2.06 | 2.05 |
| $^3A''(\mathrm{V}; n \rightarrow \pi^\star)$ | (3,4) | (1,1) | 1.85 | 1.81 |

[a]All calculations using reference (8e,7o) active space including valence $\pi$ and $n_{\mathrm{O}}$ orbitals.

Table S38: NEVPT2/aug-cc-pVTZ vertical transition energies (in eV) of triazine.

| State | Active space $(a_1, b_1, b_2, a_2)$ | State average $(A_1, B_1, B_2, A_2)$ | CASSCF | NEVPT2 |
|---|---|---|---|---|
| $^1A_1''(\mathrm{V}; n \rightarrow \pi^\star)$ | (2,4,1,2) | (1,2,0,2) | $5.88^a$ | $4.61^a$ |
| $^1A_2''(\mathrm{V}; n \rightarrow \pi^\star)$ | (2,4,1,2) | (1,1,0,0) | $5.14^a$ | $4.89^a$ |
| $^1E''(\mathrm{V}; n \rightarrow \pi^\star)$ | (2,4,1,2) | (1,2,0,2) | $5.51^a$ | $4.88^a$ |
| $^1A_2'(\mathrm{V}; \pi \rightarrow \pi^\star)$ | (0,6,0,3) | (1,0,1,0) | $5.55^d$ | $6.10^b$,$6.15^c$,$5.95^d$ |
| $^1A_1'(\mathrm{V}; \pi \rightarrow \pi^\star)$ | (0,6,0,3) | (2,0,0,0) | $8.20^d$ | $7.06^b$,$7.30^d$ |
| $^1E'(\mathrm{R}; n \rightarrow 3s)$ | (3,4,1,2) | (2,0,2,0) | $6.15^c$ | $7.45^c$ |
| $^1E''(\mathrm{V}; n \rightarrow \pi^\star)$ | (2,4,1,2) | (1,1,0,1) | $8.26^a$ | $7.98^a$ |
| $^1E'(\mathrm{V}; \pi \rightarrow \pi^\star)$ | (0,6,0,3) | (4,0,3,0) | $10.03^d$ | $7.74^b$,$8.34^d$ |
| $^3A_2''(\mathrm{V}; n \rightarrow \pi^\star)$ | (2,4,1,2) | (1,1,0,0) | $4.74^a$ | $4.51^a$ |
| $^3E''(\mathrm{V}; n \rightarrow \pi^\star)$ | (2,4,1,2) | (1,2,0,2) | $5.14^a$ | $4.61^a$ |
| $^3A_1''(\mathrm{V}; n \rightarrow \pi^\star)$ | (2,4,1,2) | (1,2,0,2) | $5.88^a$ | $4.71^a$ |
| $^3A_1'(\mathrm{V}; \pi \rightarrow \pi^\star)$ | (0,6,0,3) | (2,0,0,0) | $4.46^d$ | $5.20^b$,$5.05^d$ |
| $^3E'(\mathrm{V}; \pi \rightarrow \pi^\star)$ | (0,6,0,3) | (3,0,1,0) | $5.57^d$ | $5.83^b$,$5.73^d$ |
| $^3A_2'(\mathrm{V}; (\pi \rightarrow \pi^\star)$ | (0,6,0,3) | (1,0,1,0) | $7.70^d$ | $5.83^b$,$6.36^d$ |

[a]Using reference (12e,9o) active space including valence $\pi$ and $n_\mathrm{N}$ orbitals. [b]Using reference (6e,6o) active space including valence $\pi$ orbitals. [c]Using reference (12e,10o) active space including valence $\pi$, $n_\mathrm{N}$ and $3s$ orbitals. [d]Using reference (6e,9o) active space including valence $\pi$ and three $3p_x$ orbitals.

# S3 Selected CI results

Table S39: Vertical excitations (in eV) for various states of the studied molecules computed with an extrapolated SCI method (exFCI). The number of determinants $N_{\text{det}}$ of the largest SCI wave functions and their corresponding excitation energies are also reported. The extrapolation error is estimated as the difference in excitation energy between the largest SCI wave function and its corresponding extrapolated value.

| Molecule | Transition | 6-31+G(d) | | | *aug*-cc-pVDZ | | |
|---|---|---|---|---|---|---|---|
| | | $N_{\text{det}}$ | SCI | exFCI | $N_{\text{det}}$ | SCI | exFCI |
| Acetone | $^1A_2(\text{V}; n \to \pi^\star)$ | 26 526 782 | 4.55 | $4.60 \pm 0.05$ | | | |
| | $^3A_2(\text{V}; n \to \pi^\star)$ | 26 553 941 | 4.22 | $4.18 \pm 0.04$ | | | |
| Acrolein | $^1A''(\text{V}; n \to \pi^\star)$ | 23 273 572 | 3.84 | $3.85 \pm 0.01$ | | | |
| | $^3A''(\text{V}; n \to \pi^\star)$ | 26 531 491 | 3.59 | $3.60 \pm 0.01$ | 15 827 189 | 3.58 | $3.51 \pm 0.07$ |
| | $^3A'(\text{V}; \pi \to \pi^\star)$ | 37 480 261 | 4.01 | $3.98 \pm 0.03$ | 15 827 189 | 4.05 | $3.96 \pm 0.09$ |
| Butadiene | $^1B_u(\text{V}; \pi \to \pi^\star)$ | 20 552 493 | 6.43 | $6.41 \pm 0.02$ | | | |
| | $^1A_u(\text{R}; \pi \to 3p)$ | 20 552 493 | 6.96 | $6.95 \pm 0.01$ | 12 521 242 | 6.72 | $6.72 \pm 0.00$ |
| | $^3B_u(\text{V}; \pi \to \pi^\star)$ | 49 847 526 | 3.40 | $3.37 \pm 0.03$ | | | |
| | $^3A_g(\text{V}; \pi \to \pi^\star)$ | | | | 17 235 280 | 6.29 | $6.21 \pm 0.08$ |
| | $^3B_g(\text{V}; \pi \to 3s)$ | 49 847 526 | 6.43 | $6.40 \pm 0.03$ | | | |
| Cyanoacetylene | $^1\Sigma^-(\text{V}; \pi \to \pi^\star)$ | 21 269 249 | 6.01 | $6.02 \pm 0.01$ | 11 023 351 | 5.93 | $5.84 \pm 0.09$ |
| | $^1\Delta(\text{V}; \pi \to \pi^\star)$ | 21 269 249 | 6.29 | $6.28 \pm 0.01$ | 11 023 351 | 6.19 | $6.14 \pm 0.05$ |
| | $^3\Sigma^+(\text{V}; \pi \to \pi^\star)$ | 18 198 954 | 4.48 | $4.45 \pm 0.03$ | 25 646 703 | 4.47 | $4.41 \pm 0.06$ |
| | $^3\Delta(\text{V}; \pi \to \pi^\star)$ | 18 198 954 | 5.35 | $5.32 \pm 0.03$ | 25 646 703 | 5.28 | $5.20 \pm 0.08$ |
| | $^1A''[\text{F}](\text{V}; \pi \to \pi^\star)$ | 104 485 975 | 3.70 | $3.67 \pm 0.03$ | 62 248 690 | 3.61 | $3.50 \pm 0.02$ |
| Cyanoformaldehyde | $^1A''(\text{V}; n \to \pi^\star)$ | 17 778 047 | 3.94 | $3.92 \pm 0.02$ | 19 020 785 | 3.93 | $3.98 \pm 0.05$ |
| | $^1A''(\text{V}; \pi \to \pi^\star)$ | 17 778 047 | 6.67 | $6.60 \pm 0.07$ | 19 020 785 | 6.57 | $6.58 \pm 0.01$ |

Continued on next page

| Molecule | Transition | 6-31+G(d) | | | *aug*-cc-pVDZ | | |
| --- | --- | --- | --- | --- | --- | --- | --- |
| | | $N_{\text{det}}$ | SCI | exFCI | $N_{\text{det}}$ | SCI | exFCI |
| | $^3A''(\text{V}; n \rightarrow \pi^\star)$ | 21 011 221 | 3.54 | $3.48 \pm 0.06$ | 48 532 729 | 3.51 | $3.52 \pm 0.01$ |
| | $^3A'(\text{V}; \pi \rightarrow \pi^\star)$ | | | | 48 5327 29 | 5.10 | $5.07 \pm 0.03$ |
| Cyanogen | $^1\Sigma_u^-(\text{V}; \pi \rightarrow \pi^\star)$ | 12 1991 55 | 6.61 | $6.58 \pm 0.03$ | 20 9495 13 | 6.52 | $6.44 \pm 0.08$ |
| | $^1\Delta_u(\text{V}; \pi \rightarrow \pi^\star)$ | 12 1991 55 | 6.89 | $6.87 \pm 0.02$ | 20 9495 13 | 6.78 | $6.74 \pm 0.04$ |
| | $^3\Sigma_u^+(\text{V}; \pi \rightarrow \pi^\star)$ | 34 1277 36 | 4.97 | $4.91 \pm 0.06$ | 25 7606 68 | 4.94 | $4.87 \pm 0.07$ |
| | $^1\Sigma_u^-[\text{F}](\text{V}; \pi \rightarrow \pi^\star)$ | 21 4163 04 | 5.36 | $5.31 \pm 0.05$ | 28 8841 38 | 5.17 | $5.26 \pm 0.09$ |
| Cyclopropenone | $^1B_1(\text{V}; n \rightarrow \pi^\star)$ | 48 8976 96 | 4.40 | $4.38 \pm 0.02$ | | | |
| | $^1A_2(\text{V}; n \rightarrow \pi^\star)$ | 24 5411 16 | 5.70 | $5.64 \pm 0.06$ | | | |
| | $^3B_1(\text{V}; n \rightarrow \pi^\star)$ | 24 008 328 | 4.07 | $4.00 \pm 0.07$ | | | |
| | $^3B_2(\text{V}; \pi \rightarrow \pi^\star)$ | 48 311 362 | 4.95 | $4.95 \pm 0.00$ | | | |
| Cyclopropenethione | $^1A_2(\text{V}; n \rightarrow \pi^\star)$ | 39 385 657 | 3.46 | $3.45 \pm 0.01$ | | | |
| | $^1B_1(\text{V}; n \rightarrow \pi^\star)$ | 39 385 657 | 3.50 | $3.44 \pm 0.05$ | | | |
| | $^1B_2(\text{V}; \pi \rightarrow \pi^\star)$ | 39 385 657 | 4.68 | $4.59 \pm 0.09$ | | | |
| | $^3A_2(\text{V}; n \rightarrow \pi^\star)$ | 23 904 962 | 3.32 | $3.29 \pm 0.03$ | | | |
| | $^3B_2(\text{V}; \pi \rightarrow \pi^\star)$ | 23 904 962 | 4.06 | $4.03 \pm 0.03$ | | | |
| Diacetylene | $^1\Sigma_u^-(\text{V}; \pi \rightarrow \pi^\star)$ | 18 955 451 | 5.58 | $5.52 \pm 0.06$ | 19 192 556 | 5.45 | $5.47 \pm 0.02$ |
| | $^1\Delta_u(\text{V}; \pi \rightarrow \pi^\star)$ | 18 955 451 | 5.85 | $5.84 \pm 0.01$ | 19 192 556 | 5.45 | $5.69 \pm 0.02$ |
| | $^3\Sigma_u^+(\text{V}; \pi \rightarrow \pi^\star)$ | 13 777 757 | 4.11 | $4.04 \pm 0.07$ | 26 668 471 | 4.11 | $4.07 \pm 0.04$ |
| | $^3\Delta_u(\text{V}; \pi \rightarrow \pi^\star)$ | 13 777 757 | 4.93 | $4.94 \pm 0.01$ | 26 668 471 | 4.87 | $4.85 \pm 0.02$ |
| Glyoxal | $^1A_u(\text{V}; n \rightarrow \pi^\star)$ | 51 656 090 | 2.96 | $2.93 \pm 0.03$ | 34 125 394 | 2.94 | $2.93 \pm 0.01$ |
| | $^1B_g(\text{V}; n \rightarrow \pi^\star)$ | 24 394 242 | 4.34 | $4.28 \pm 0.06$ | | | |

Continued on next page

| Molecule | Transition | 6-31+G(d) | | | *aug*-cc-pVDZ | | |
|---|---|---|---|---|---|---|---|
| | | $N_{\text{det}}$ | SCI | exFCI | $N_{\text{det}}$ | SCI | exFCI |
| | $^3A_u(\text{V}; n \to \pi^\star)$ | 47 693 908 | 2.58 | $2.54 \pm 0.04$ | | | |
| Isobutene | $^1B_1(\text{R}; \pi \to 3s)$ | 28 095 377 | 6.86 | $6.78 \pm 0.08$ | | | |
| | $^1A_1(\text{R}; \pi \to 3p)$ | 59 728 169 | 7.22 | $7.16 \pm 0.02$ | | | |
| | $^3A_1\text{V}; (\pi \to \pi^\star)$ | 32 440 621 | 4.54 | $4.56 \pm 0.02$ | | | |
| Methylenecyclopropene | $^1B_2(\text{V}; \pi \to \pi^\star)$ | 51 918 524 | 4.35 | $4.32 \pm 0.03$ | | | |
| | $^1A_2(\text{R}; \pi \to 3p)$ | 25 146 911 | 6.02 | $5.92 \pm 0.10$ | | | |
| | $^1A_1(\text{V}; \pi \to \pi^\star)$ | 31 721 213 | 6.21 | $6.20 \pm 0.01$ | | | |
| | $^3B_2(\text{V}; \pi \to \pi^\star)$ | 24 379 551 | 3.50 | $3.44 \pm 0.06$ | 43 090 114 | 3.49 | $3.45 \pm 0.04$ |
| | $^3A_1(\text{V}; \pi \to \pi^\star)$ | 24 379 551 | 4.77 | $4.67 \pm 0.10$ | 43 090 114 | 4.77 | $4.79 \pm 0.02$ |
| Propynal | $^1A''(\text{V}; n \to \pi^\star)$ | 48 945 252 | 3.90 | $3.84 \pm 0.06$ | 28 249 344 | 3.92 | $3.89 \pm 0.03$ |
| | $^1A''(\text{V}; \pi \to \pi^\star)$ | 26 554 616 | 5.72 | $5.64 \pm 0.08$ | 28 249 344 | 5.72 | $5.63 \pm 0.09$ |
| | $^3A''(\text{V}; n \to \pi^\star)$ | 23 182 284 | 3.58 | $3.54 \pm 0.04$ | | | |
| | $^3A'(\text{V}; \pi \to \pi^\star)$ | 39 375 360 | 4.52 | $4.44 \pm 0.08$ | | | |
| Thioacetone | $^1A_2(\text{V}; n \to \pi^\star)$ | 26 515 070 | 2.56 | $2.61 \pm 0.05$ | | | |
| | $^3A_2(\text{V}; n \to \pi^\star)$ | 63 669 401 | 2.36 | $2.36 \pm 0.00$ | | | |
| Thiopropynal | $^1A''(\text{V}; n \to \pi^\star)$ | 15 782 429 | 2.07 | $2.08 \pm 0.01$ | | | |

# S4 Benchmarks

## S4.1 Raw data

Table S40: Comparisons between the TBE(FC)/*aug*-cc-pVTZ benchmark (see Table 11) and the results obtained with various computational approaches using the same basis set. STEOM stands for STEOM-CCSD and CC(3) for CCSDR(3).

| Compound | State | TBE | CIS(D) | CC2 | CCSD | STEOM | CC(3) | CCSDT-3 | CC3 | ADC(2) |
|---|---|---|---|---|---|---|---|---|---|---|
| Acetone | $^1A_2(\text{V}; n \to \pi^\star)$ | 4.47 | 4.51 | 4.55 | 4.54 | 4.40 | 4.48 | 4.49 | 4.48 | 4.37 |
| | $^1B_2(\text{R}; n \to 3s)$ | 6.46 | 5.91 | 5.91 | 6.59 | 6.62 | 6.46 | 6.50 | 6.43 | 5.87 |
| | $^1A_2(\text{R}; n \to 3p)$ | 7.47 | 6.83 | 6.84 | 7.57 | | 7.47 | 7.51 | 7.45 | 6.81 |
| | $^1A_1(\text{R}; n \to 3p)$ | 7.51 | 7.04 | 6.89 | 7.63 | 7.68 | 7.52 | 7.55 | 7.48 | 6.85 |
| | $^1B_2(\text{R}; n \to 3p)$ | 7.62 | 6.93 | 7.02 | 7.72 | | 7.61 | 7.65 | 7.59 | 6.99 |
| | $^3A_2(\text{V}; n \to \pi^\star)$ | 4.13 | 4.15 | 4.16 | 4.15 | 4.05 | | | 4.15 | 4.00 |
| | $^3A_1(\text{V}; \pi \to \pi^\star)$ | 6.25 | 6.50 | 6.50 | 6.19 | 6.05 | | | 6.28 | 6.37 |
| Acrolein | $^1A''(\text{V}; n \to \pi^\star)$ | 3.78 | 3.89 | 3.85 | 3.91 | 3.85 | 3.80 | 3.78 | 3.74 | 3.68 |
| | $^1A'(\text{V}; \pi \to \pi^\star)$ | 6.69 | 6.88 | 6.80 | 6.87 | | 6.69 | 6.71 | 6.65 | 6.74 |
| | $^1A''(\text{V}; n \to \pi^\star)$ | *6.72* | 7.76 | 6.68 | 7.27 | 6.98 | 6.94 | 6.89 | 6.75 | 6.59 |
| | $^1A'(\text{R}; n \to 3s)$ | 7.08 | 6.92 | 6.40 | 7.24 | 7.25 | 7.12 | 7.15 | 7.07 | 6.35 |
| | $^3A''(\text{V}; n \to \pi^\star)$ | 3.51 | 3.56 | 3.49 | 3.55 | 3.48 | | | 3.46 | 3.33 |
| | $^3A'(\text{V}; \pi \to \pi^\star)$ | 3.94 | 4.14 | 4.06 | 3.88 | 3.72 | | | 3.94 | 4.05 |
| | $^3A'(\text{V}; \pi \to \pi^\star)$ | 6.18 | 6.42 | 6.37 | 6.14 | 6.00 | | | 6.19 | 6.31 |
| | $^3A''(\text{V}; n \to \pi^\star)$ | *6.54* | | 6.55 | 7.09 | | | | 6.61 | 6.47 |
| Benzene | $^1B_{2u}(\text{V}; \pi \to \pi^\star)$ | 5.06 | 5.32 | 5.26 | 5.20 | 5.01 | 5.14 | 5.11 | 5.09 | 5.27 |
| | $^1B_{1u}(\text{V}; \pi \to \pi^\star)$ | 6.45 | 6.61 | 6.48 | 6.50 | 6.51 | 6.47 | 6.45 | 6.44 | 6.45 |
| | $^1E_{1g}(\text{R}; \pi \to 3s)$ | 6.52 | 6.57 | 6.47 | 6.58 | 6.65 | 6.54 | 6.54 | 6.52 | 6.52 |
| | $^1A_{2u}(\text{R}; \pi \to 3p)$ | 7.08 | 7.08 | 7.00 | 7.12 | 7.17 | 7.10 | 7.09 | 7.08 | 7.06 |
| | $^1E_{2u}(\text{R}; \pi \to 3p)$ | 7.15 | 7.14 | 7.06 | 7.20 | | 7.17 | 7.16 | 7.15 | 7.12 |
| | $^3B_{1u}(\text{V}; \pi \to \pi^\star)$ | 4.16 | 4.47 | 4.37 | 4.00 | | | | 4.18 | 4.37 |
| | $^3E_{1u}(\text{V}; \pi \to \pi^\star)$ | 4.85 | 5.12 | 5.08 | 4.93 | 4.88 | | | 4.86 | 5.07 |
| | $^3B_{2u}(\text{V}; \pi \to \pi^\star)$ | 5.81 | 5.95 | 5.89 | 5.77 | 5.78 | | | 5.81 | 5.87 |
| Butadiene | $^1B_u(\text{V}; \pi \to \pi^\star)$ | 6.22 | 6.24 | 6.16 | 6.35 | 6.33 | 6.21 | 6.24 | 6.22 | 6.12 |
| | $^1B_g(\text{R}; \pi \to 3s)$ | 6.33 | 6.34 | 6.26 | 6.40 | 6.38 | 6.33 | 6.34 | 6.33 | 6.31 |
| | $^1A_g(\text{V}; \pi \to \pi^\star)$ | 6.50 | 7.35 | 7.09 | 7.12 | | 6.86 | 6.76 | 6.67 | 7.14 |
| | $^1A_u(\text{R}; \pi \to 3p)$ | 6.64 | 6.65 | 6.57 | 6.71 | 6.69 | 6.65 | 6.66 | 6.64 | 6.63 |
| | $^1A_u(\text{R}; \pi \to 3p)$ | 6.80 | 6.78 | 6.70 | 6.87 | 6.92 | 6.80 | 6.81 | 6.80 | 6.76 |
| | $^1B_u(\text{R}; \pi \to 3p)$ | 7.68 | 7.71 | 7.63 | 7.76 | 7.76 | 7.68 | | 7.68 | 7.48 |
| | $^3B_u(\text{V}; \pi \to \pi^\star)$ | 3.36 | 3.55 | 3.45 | 3.29 | 3.17 | | | 3.36 | 3.46 |
| | $^3A_g(\text{V}; \pi \to \pi^\star)$ | 5.20 | 5.33 | 5.30 | 5.17 | 5.03 | | | 5.20 | 5.27 |
| | $^3B_g(\text{R}; \pi \to 3s)$ | 6.29 | 6.31 | 6.21 | 6.33 | 6.42 | | | 6.28 | 6.27 |
| Cyanoacetylene | $^1\Sigma^-(\text{V}; \pi \to \pi^\star)$ | 5.80 | 6.14 | 6.03 | 5.88 | 5.87 | 5.84 | 5.81 | 5.80 | 5.99 |

Continued on next page

| Compound | State | TBE | CIS(D) | CC2 | CCSD | STEOM | CC(3) | CCSDT-3 | CC3 | ADC(2) |
|---|---|---|---|---|---|---|---|---|---|---|
| | $^1\Delta$(V; $\pi \to \pi^\star$) | 6.07 | 6.41 | 6.30 | 6.15 | 6.20 | 6.11 | 6.09 | 6.08 | 6.25 |
| | $^3\Sigma^+$(V; $\pi \to \pi^\star$) | 4.44 | 4.89 | 4.80 | 4.38 | 4.35 | | | 4.45 | 4.77 |
| | $^3\Delta$(V; $\pi \to \pi^\star$) | 5.21 | 5.60 | 5.50 | 5.24 | 5.22 | | | 5.22 | 5.46 |
| | $^1A''$[F](V; $\pi \to \pi^\star$) | 3.54 | 3.83 | 3.79 | 3.58 | 3.52 | 3.58 | 3.54 | 3.54 | 3.63 |
| Cyanoformaldehyde | $^1A''$(V; $n \to \pi^\star$) | 3.81 | 3.98 | 3.97 | 3.94 | 3.80 | 3.87 | 3.86 | 3.83 | 3.83 |
| | $^1A''$(V; $\pi \to \pi^\star$) | 6.46 | 7.10 | 6.74 | 6.67 | 6.56 | 6.50 | 6.47 | 6.42 | 6.73 |
| | $^3A''$(V; $n \to \pi^\star$) | 3.44 | 3.54 | 3.51 | 3.49 | 3.42 | | | 3.46 | 3.37 |
| | $^3A'$(V; $\pi \to \pi^\star$) | 5.01 | 5.43 | 5.34 | 4.97 | 4.89 | | | 5.01 | 5.27 |
| Cyanogen | $^1\Sigma_u^-$(V; $\pi \to \pi^\star$) | 6.39 | 6.85 | 6.72 | 6.50 | 6.46 | 6.44 | 6.40 | 6.39 | 6.67 |
| | $^1\Delta_u$(V; $\pi \to \pi^\star$) | 6.66 | 7.15 | 7.02 | 6.78 | 6.80 | 6.72 | 6.68 | 6.66 | 6.95 |
| | $^3\Sigma_u^+$(V; $\pi \to \pi^\star$) | 4.91 | 5.44 | 5.35 | 4.84 | 4.81 | | | 4.90 | 5.31 |
| | $^1\Sigma_u^-$[F](V; $\pi \to \pi^\star$) | 5.05 | 5.61 | 5.48 | 5.13 | 5.07 | 5.14 | 5.06 | 5.06 | 5.39 |
| Cyclopentadiene | $^1B_2$(V; $\pi \to \pi^\star$) | 5.56 | 5.62 | 5.52 | 5.67 | 5.59 | 5.53 | 5.56 | 5.54 | 5.49 |
| | $^1A_2$(R; $\pi \to 3s$) | 5.78 | 5.75 | 5.66 | 5.83 | 5.80 | 5.78 | 5.78 | 5.77 | 5.71 |
| | $^1B_1$(R; $\pi \to 3p$) | 6.41 | 6.33 | 6.26 | 6.45 | 6.44 | 6.41 | 6.41 | 6.40 | 6.31 |
| | $^1A_2$(R; $\pi \to 3p$) | 6.46 | 6.37 | 6.30 | 6.50 | 6.60 | 6.46 | 6.46 | 6.45 | 6.35 |
| | $^1B_2$(R; $\pi \to 3p$) | 6.56 | 6.50 | 6.42 | 6.61 | 6.65 | 6.57 | 6.56 | 6.56 | 6.48 |
| | $^1A_1$(V; $\pi \to \pi^\star$) | *6.52* | 7.63 | 6.86 | 6.96 | | 6.71 | 6.66 | 6.57 | 6.91 |
| | $^3B_2$(V; $\pi \to \pi^\star$) | 3.31 | 3.52 | 3.42 | 3.24 | 3.11 | | | 3.32 | 3.42 |
| | $^3A_1$(V; $\pi \to \pi^\star$) | 5.11 | 5.30 | 5.36 | 5.09 | 4.79 | | | 5.12 | 5.23 |
| | $^3A_2$(R; $\pi \to 3s$) | 5.73 | 5.73 | 5.62 | 5.78 | 5.86 | | | 5.73 | 5.67 |
| | $^3B_1$(R; $\pi \to 3p$) | 6.36 | 6.31 | 6.22 | 6.40 | 6.47 | | | 6.36 | 6.27 |
| Cyclopropenone | $^1B_1$(V; $n \to \pi^\star$) | 4.26 | 4.27 | 4.01 | 4.53 | 4.18 | 4.28 | 4.31 | 4.21 | 3.88 |
| | $^1A_2$(V; $n \to \pi^\star$) | 5.55 | 5.65 | 5.65 | 5.40 | | 5.59 | 5.59 | 5.57 | 5.47 |
| | $^1B_2$(R; $n \to 3s$) | 6.34 | 6.32 | 5.84 | 6.44 | 6.36 | 6.35 | 6.38 | 6.32 | 5.79 |
| | $^1B_2$(V; $\pi \to \pi^\star$) | 6.54 | 6.60 | 6.46 | 6.82 | | 6.59 | 6.61 | 6.54 | 6.33 |
| | $^1B_2$(R; $n \to 3p$) | 6.98 | 6.48 | 6.56 | 7.09 | 7.07 | 6.98 | | 6.96 | 6.43 |
| | $^1A_1$(R; $n \to 3p$) | 7.02 | 6.54 | 6.47 | 7.12 | | 7.02 | 7.06 | 7.00 | 6.41 |
| | $^1A_1$(V; $\pi \to \pi^\star$) | 8.28 | 8.22 | 8.28 | 8.35 | 8.19 | 8.29 | | 8.28 | 8.10 |
| | $^3B_1$(V; $n \to \pi^\star$) | 3.93 | 4.15 | 3.73 | 4.18 | 4.13 | | | 3.91 | 3.62 |
| | $^3B_2$(V; $\pi \to \pi^\star$) | 4.88 | 5.26 | 4.99 | 4.91 | 4.88 | | | 4.89 | 4.90 |
| | $^3A_2$(V; $n \to \pi^\star$) | 5.35 | 5.96 | 5.45 | 5.40 | 5.01 | | | 5.37 | 5.28 |
| | $^3A_1$(V; $\pi \to \pi^\star$) | 6.79 | 6.97 | 7.02 | 6.76 | 6.39 | | | 6.83 | 6.84 |
| Cyclopropenethione | $^1A_2$(V; $n \to \pi^\star$) | 3.41 | 3.45 | 3.53 | 3.51 | 3.34 | 3.43 | 3.46 | 3.43 | 3.38 |
| | $^1B_1$(V; $n \to \pi^\star$) | 3.45 | 3.56 | 3.50 | 3.84 | | 3.51 | 3.56 | 3.43 | 3.37 |
| | $^1B_2$(V; $\pi \to \pi^\star$) | 4.60 | 5.06 | 4.91 | 4.98 | | 4.69 | 4.73 | 4.64 | 4.72 |
| | $^1B_2$(R; $n \to 3s$) | 5.34 | 5.24 | 5.22 | 5.41 | 5.45 | 5.34 | 5.38 | 5.34 | 5.17 |
| | $^1A_1$(V; $\pi \to \pi^\star$) | 5.46 | 5.47 | 5.59 | 5.55 | | 5.48 | 5.52 | 5.49 | 5.36 |
| | $^1B_2$(R; $n \to 3p$) | 5.92 | 5.93 | 5.82 | 6.03 | 6.05 | 5.93 | 5.97 | 5.93 | 5.77 |

Continued on next page

| Compound | State | TBE | CIS(D) | CC2 | CCSD | STEOM | CC(3) | CCSDT-3 | CC3 | ADC(2) |
|---|---|---|---|---|---|---|---|---|---|---|
| | $^3A_2(\mathrm{V}; n \to \pi^\star)$ | 3.28 | 3.34 | 3.37 | 3.34 | 3.23 | | | 3.30 | 3.23 |
| | $^3B_1(\mathrm{V}; n \to \pi^\star)$ | 3.32 | 3.55 | 3.38 | 3.69 | 3.55 | | | 3.31 | 3.26 |
| | $^3B_2(\mathrm{V}; \pi \to \pi^\star)$ | 4.01 | 4.62 | 4.24 | 4.16 | 4.05 | | | 4.02 | 4.12 |
| | $^3A_1(\mathrm{V}; \pi \to \pi^\star)$ | 4.01 | 4.12 | 4.16 | 3.97 | 3.87 | | | 4.03 | 4.04 |
| Diacetylene | $^1\Sigma_u^-(\mathrm{V}; \pi \to \pi^\star)$ | 5.33 | 5.62 | 5.51 | 5.41 | 5.37 | 5.37 | 5.35 | 5.34 | 5.49 |
| | $^1\Delta_u(\mathrm{V}; \pi \to \pi^\star)$ | 5.61 | 5.86 | 5.76 | 5.67 | 5.64 | 5.64 | 5.62 | 5.61 | 5.72 |
| | $^3\Sigma_u^+(\mathrm{V}; \pi \to \pi^\star)$ | 4.10 | 4.48 | 4.39 | 4.01 | 4.05 | | | 4.08 | 4.37 |
| | $^3\Delta_u(\mathrm{V}; \pi \to \pi^\star)$ | 4.78 | 5.14 | 5.03 | 4.82 | 4.87 | | | 4.80 | 5.01 |
| Furan | $^1A_2(\mathrm{R}; \pi \to 3s)$ | 6.09 | 6.16 | 6.06 | 6.17 | 6.15 | 6.10 | 6.09 | 6.08 | 6.12 |
| | $^1B_2(\mathrm{V}; \pi \to \pi^\star)$ | 6.37 | 6.59 | 6.45 | 6.51 | 6.45 | 6.38 | 6.37 | 6.34 | 6.47 |
| | $^1A_1(\mathrm{V}; \pi \to \pi^\star)$ | 6.56 | 7.01 | 6.77 | 6.85 | | 6.68 | 6.65 | 6.58 | 6.76 |
| | $^1B_1(\mathrm{R}; \pi \to 3p)$ | 6.64 | 6.67 | 6.59 | 6.71 | 6.70 | 6.65 | 6.64 | 6.63 | 6.64 |
| | $^1A_2(\mathrm{R}; \pi \to 3p)$ | 6.81 | 6.84 | 6.75 | 6.89 | 6.93 | 6.82 | 6.81 | 6.80 | 6.82 |
| | $^1B_2(\mathrm{R}; \pi \to 3p)$ | 7.24 | 7.34 | 7.25 | 7.32 | 7.35 | 7.25 | | 7.23 | 7.29 |
| | $^3B_2(\mathrm{V}; \pi \to \pi^\star)$ | 4.20 | 4.51 | 4.43 | 4.15 | 4.17 | | | 4.22 | 4.41 |
| | $^3A_1(\mathrm{V}; \pi \to \pi^\star)$ | 5.46 | 5.69 | 5.66 | 5.47 | 5.61 | | | 5.48 | 5.59 |
| | $^3A_2(\mathrm{R}; \pi \to 3s)$ | 6.02 | 6.13 | 6.01 | 6.11 | 6.20 | | | 6.02 | 6.08 |
| | $^3B_1(\mathrm{R}; \pi \to 3p)$ | 6.59 | 6.64 | 6.55 | 6.66 | 6.73 | | | 6.59 | 6.61 |
| Glyoxal | $^1A_u(\mathrm{V}; n \to \pi^\star)$ | 2.88 | 3.01 | 2.91 | 3.01 | 2.86 | 2.92 | 2.91 | 2.88 | 2.83 |
| | $^1B_g(\mathrm{V}; n \to \pi^\star)$ | 4.24 | 4.46 | 4.44 | 4.42 | 4.32 | 4.32 | 4.30 | 4.27 | 4.27 |
| | $^1A_g(\mathrm{V}; n, n \to \pi^\star, \pi^\star)$ | 5.61 | | | | | | 7.26 | 6.76 | |
| | $^1B_g(\mathrm{V}; n \to \pi^\star)$ | 6.57 | 7.01 | 6.51 | 7.12 | | 6.75 | 6.73 | 6.58 | 6.50 |
| | $^1B_u(\mathrm{R}; n \to 3p)$ | 7.71 | 7.25 | 7.16 | 7.84 | 7.94 | 7.71 | 7.74 | 7.67 | 7.18 |
| | $^3A_u(\mathrm{V}; n \to \pi^\star)$ | 2.49 | 2.59 | 2.47 | 2.56 | 2.44 | | | 2.49 | 2.39 |
| | $^3B_g(\mathrm{V}; n \to \pi^\star)$ | 3.89 | 4.00 | 3.96 | 3.96 | 3.88 | | | 3.90 | 3.82 |
| | $^3B_u(\mathrm{V}; \pi \to \pi^\star)$ | 5.15 | 5.47 | 5.42 | 5.10 | 4.92 | | | 5.17 | 5.33 |
| | $^3A_g(\mathrm{V}; \pi \to \pi^\star)$ | 6.30 | 6.54 | 6.56 | 6.23 | 6.13 | | | 6.30 | 6.45 |
| Imidazole | $^1A''(\mathrm{R}; \pi \to 3s)$ | 5.71 | 5.81 | 5.69 | 5.80 | 5.91 | 5.73 | 5.72 | 5.71 | 5.75 |
| | $^1A'(\mathrm{V}; \pi \to \pi^\star)$ | 6.41 | 6.73 | 6.51 | 6.59 | 6.76 | 6.47 | 6.46 | 6.41 | 6.50 |
| | $^1A''(\mathrm{V}; n \to \pi^\star)$ | 6.50 | 6.52 | 6.47 | 6.58 | 6.66 | 6.53 | 6.51 | 6.50 | 6.51 |
| | $^1A'(\mathrm{R}; \pi \to 3p)$ | *6.83* | 7.40 | 6.41 | 7.02 | 6.92 | 6.93 | 6.91 | 6.87 | |
| | $^3A'(\mathrm{V}; \pi \to \pi^\star)$ | 4.73 | 5.04 | 4.94 | 4.68 | 4.66 | | | 4.75 | 4.92 |
| | $^3A''(\mathrm{R}; \pi \to 3s)$ | 5.66 | 5.80 | 5.66 | 5.77 | 5.87 | | | 5.67 | 5.72 |
| | $^3A'(\mathrm{V}; \pi \to \pi^\star)$ | 5.74 | 6.06 | 5.94 | 5.77 | 5.60 | | | 5.74 | 5.93 |
| | $^3A''(\mathrm{V}; n \to \pi^\star)$ | 6.31 | 6.47 | 6.36 | 6.40 | 6.28 | | | 6.33 | 6.31 |
| Isobutene | $^1B_1(\mathrm{R}; \pi \to 3s)$ | 6.46 | 6.46 | 6.37 | 6.54 | 6.59 | 6.46 | 6.47 | 6.45 | 6.43 |
| | $^1A_1(\mathrm{R}; \pi \to 3p)$ | 7.01 | 7.01 | 6.95 | 7.09 | 7.11 | 7.00 | 7.01 | 7.00 | 6.97 |
| | $^3A_1(\mathrm{V}; (\pi \to \pi^\star)$ | 4.53 | 4.68 | 4.62 | 4.48 | 4.22 | | | 4.53 | 4.62 |
| Methylenecyclopropene | $^1B_2(\mathrm{V}; \pi \to \pi^\star)$ | 4.28 | 4.72 | 4.51 | 4.58 | 4.76 | 4.35 | 4.38 | 4.31 | 4.46 |

Continued on next page

| Compound | State | TBE | CIS(D) | CC2 | CCSD | STEOM | CC(3) | CCSDT-3 | CC3 | ADC(2) |
|---|---|---|---|---|---|---|---|---|---|---|
| | $^1B_1$(R; $\pi \rightarrow 3s$) | 5.44 | 5.43 | 5.35 | 5.48 | 5.45 | 5.44 | 5.45 | 5.44 | 5.38 |
| | $^1A_2$(R; $\pi \rightarrow 3p$) | 5.96 | 5.94 | 5.85 | 6.00 | 6.01 | 5.96 | 5.97 | 5.95 | 5.87 |
| | $^1A_1$(V; $\pi \rightarrow \pi^\star$) | *6.12* | 6.14 | 6.09 | 6.18 | 6.21 | 6.12 | 6.14 | 6.13 | 6.09 |
| | $^3B_2$(V; $\pi \rightarrow \pi^\star$) | 3.49 | 3.94 | 3.64 | 3.57 | 3.67 | | | 3.50 | 3.61 |
| | $^3A_1$(V; $\pi \rightarrow \pi^\star$) | 4.74 | 4.86 | 4.81 | 4.69 | 4.78 | | | 4.74 | 4.80 |
| Propynal | $^1A''$(V; $n \rightarrow \pi^\star$) | 3.80 | 3.95 | 3.96 | 3.84 | 3.82 | 3.86 | 3.85 | 3.82 | 3.78 |
| | $^1A''$(V; $\pi \rightarrow \pi^\star$) | 5.54 | 5.95 | 5.71 | 5.69 | 5.72 | 5.57 | 5.55 | 5.51 | 5.73 |
| | $^3A''$(V; $n \rightarrow \pi^\star$) | 3.47 | 3.55 | 3.53 | 3.53 | 3.40 | | | 3.49 | 3.38 |
| | $^3A'$(V; $\pi \rightarrow \pi^\star$) | 4.47 | 4.81 | 4.71 | 4.40 | 4.38 | | | 4.43 | 4.67 |
| Pyrazine | $^1B_{3u}$(V; $n \rightarrow \pi^\star$) | 4.15 | 4.37 | 4.14 | 4.32 | 4.10 | 4.21 | 4.20 | 4.14 | 4.17 |
| | $^1A_u$(V; $n \rightarrow \pi^\star$) | 4.98 | 4.91 | 4.86 | 5.23 | 5.04 | 5.04 | 5.06 | 4.97 | 4.88 |
| | $^1B_{2u}$(V; $\pi \rightarrow \pi^\star$) | 5.02 | 5.26 | 5.14 | 5.15 | 4.83 | 5.09 | 5.06 | 5.03 | 5.17 |
| | $^1B_{2g}$(V; $n \rightarrow \pi^\star$) | 5.71 | 6.22 | 5.86 | 6.00 | 5.71 | 5.84 | 5.80 | 5.71 | 5.87 |
| | $^1A_g$(R; $n \rightarrow 3s$) | 6.65 | 6.20 | 6.20 | 6.83 | 6.86 | 6.71 | 6.74 | 6.66 | 6.30 |
| | $^1B_{1g}$(V; $n \rightarrow \pi^\star$) | 6.74 | 7.31 | 6.67 | 7.14 | 7.33 | 6.85 | 6.87 | 6.73 | 6.67 |
| | $^1B_{1u}$(V; $\pi \rightarrow \pi^\star$) | 6.88 | 7.13 | 6.89 | 6.96 | | 6.90 | 6.88 | 6.86 | 6.88 |
| | $^1B_{1g}$(R; $\pi \rightarrow 3s$) | 7.21 | 7.31 | 7.21 | 7.26 | | 7.22 | 7.21 | 7.20 | 7.27 |
| | $^1B_{2u}$(R; $n \rightarrow 3p$) | 7.24 | 7.30 | 6.74 | 7.44 | 7.49 | 7.31 | 7.35 | 7.25 | |
| | $^1B_{1u}$(R; $n \rightarrow 3p$) | 7.44 | 7.19 | 7.03 | 7.60 | | 7.50 | 7.52 | 7.45 | |
| | $^1B_{1u}$(V; $\pi \rightarrow \pi^\star$) | *7.98* | 7.85 | 7.87 | 8.20 | | 7.98 | 8.02 | 7.94 | |
| | $^3B_{3u}$(V; $n \rightarrow \pi^\star$) | 3.59 | 3.84 | 3.60 | 3.70 | 3.48 | | | 3.59 | 3.62 |
| | $^3B_{1u}$(V; $\pi \rightarrow \pi^\star$) | 4.35 | 4.76 | 4.60 | 4.19 | 3.93 | | | 4.39 | 4.57 |
| | $^3B_{2u}$(V; $(\pi \rightarrow \pi^\star$) | 4.39 | 4.67 | 4.57 | 4.40 | 4.32 | | | 4.40 | 4.59 |
| | $^3A_u$(V; $n \rightarrow \pi^\star$) | 4.93 | 4.93 | 4.82 | 5.16 | 4.97 | | | 4.93 | 4.84 |
| | $^3B_{2g}$(V; $n \rightarrow \pi^\star$) | 5.08 | 5.41 | 5.17 | 5.21 | 4.89 | | | 5.08 | |
| | $^3B_{1u}$(V; $\pi \rightarrow \pi^\star$) | 5.28 | 5.59 | 5.59 | 5.35 | 5.21 | | | 5.29 | |
| Pyridazine | $^1B_1$(V; $n \rightarrow \pi^\star$) | 3.83 | 4.12 | 3.78 | 4.03 | 3.76 | 3.91 | 3.89 | 3.83 | 3.79 |
| | $^1A_2$(V; $n \rightarrow \pi^\star$) | 4.37 | 4.84 | 4.26 | 4.65 | 4.44 | 4.46 | 4.47 | 4.37 | 4.27 |
| | $^1A_1$(V; $\pi \rightarrow \pi^\star$) | 5.26 | 5.51 | 5.43 | 5.43 | | 5.36 | 5.32 | 5.29 | 5.44 |
| | $^1A_2$(V; $n \rightarrow \pi^\star$) | 5.72 | 5.62 | 5.79 | 6.01 | 5.76 | 5.84 | 5.82 | 5.74 | 5.81 |
| | $^1B_2$(R; $n \rightarrow 3s$) | 6.17 | 5.83 | 5.59 | 6.42 | 6.45 | 6.27 | 6.31 | 6.17 | 5.69 |
| | $^1B_1$(V; $n \rightarrow \pi^\star$) | 6.37 | 6.39 | 6.33 | 6.67 | 6.47 | 6.46 | 6.47 | 6.37 | 6.35 |
| | $^1B_2$(V; $\pi \rightarrow \pi^\star$) | 6.75 | | 6.86 | 6.88 | | 6.81 | 6.77 | 6.74 | 6.85 |
| | $^3B_1$(V; $n \rightarrow \pi^\star$) | 3.19 | 3.50 | 3.18 | 3.30 | 3.06 | | | 3.19 | 3.19 |
| | $^3A_2$(V; $n \rightarrow \pi^\star$) | 4.11 | 4.64 | 4.01 | 4.31 | 4.13 | | | 4.11 | 4.02 |
| | $^3B_2$(V; $\pi \rightarrow \pi^\star$) | *4.34* | 4.75 | 4.61 | 4.17 | 3.89 | | | 4.38 | 4.60 |
| | $^3A_1$(V; $\pi \rightarrow \pi^\star$) | 4.82 | 5.18 | 5.07 | 4.86 | 4.78 | | | 4.83 | 5.06 |
| Pyridine | $^1B_1$(V; $n \rightarrow \pi^\star$) | 4.95 | 5.22 | 4.99 | 5.17 | 4.94 | 5.04 | 5.03 | 4.96 | 4.98 |
| | $^1B_2$(V; $\pi \rightarrow \pi^\star$) | 5.14 | 5.40 | 5.32 | 5.29 | 5.03 | 5.23 | 5.20 | 5.17 | 5.33 |

Continued on next page

| Compound | State | TBE | CIS(D) | CC2 | CCSD | STEOM | CC(3) | CCSDT-3 | CC3 | ADC(2) |
|---|---|---|---|---|---|---|---|---|---|---|
| | $^1A_2(\mathrm{V}; n \to \pi^\star)$ | 5.40 | 5.33 | 5.28 | 5.64 | 5.45 | 5.46 | 5.48 | 5.40 | 5.27 |
| | $^1A_1(\mathrm{V}; \pi \to \pi^\star)$ | 6.62 | 6.84 | 6.24 | 6.96 | 6.98 | 6.67 | 6.65 | 6.63 | 6.31 |
| | $^1A_1(\mathrm{R}; n \to 3s)$ | 6.76 | 6.38 | 6.68 | 6.71 | | 6.83 | 6.86 | 6.76 | 6.65 |
| | $^1A_2(\mathrm{R}; \pi \to 3s)$ | 6.82 | 6.88 | 6.79 | 6.87 | 6.94 | 6.83 | 6.83 | 6.81 | 6.83 |
| | $^1B_2(\mathrm{V}; \pi \to \pi^\star)$ | *7.40* | 7.56 | 7.37 | 7.55 | | 7.40 | | 7.38 | 6.87 |
| | $^1B_1(\mathrm{R}; \pi \to 3p)$ | 7.38 | 7.42 | 7.34 | 7.43 | 7.49 | 7.40 | 7.40 | 7.38 | 7.38 |
| | $^1A_1(\mathrm{V}; \pi \to \pi^\star)$ | 7.39 | 7.56 | 7.45 | 7.59 | | 7.44 | 7.47 | 7.39 | 7.48 |
| | $^3A_1(\mathrm{V}; \pi \to \pi^\star)$ | 4.30 | 4.66 | 4.53 | 4.15 | 3.93 | | | 4.33 | 4.53 |
| | $^3B_1(\mathrm{V}; n \to \pi^\star)$ | 4.46 | 4.72 | 4.48 | 4.59 | 4.41 | | | 4.46 | 4.47 |
| | $^3B_2(\mathrm{V}; \pi \to \pi^\star)$ | 4.79 | 5.08 | 4.98 | 4.83 | 4.78 | | | 4.79 | 4.98 |
| | $^3A_1(\mathrm{V}; \pi \to \pi^\star)$ | 5.04 | 5.33 | 5.29 | 5.11 | 5.03 | | | 5.05 | 5.28 |
| | $^3A_2(\mathrm{V}; n \to \pi^\star)$ | 5.36 | 5.36 | 5.24 | 5.58 | 5.39 | | | 5.35 | 5.23 |
| | $^3B_2(\mathrm{V}; \pi \to \pi^\star)$ | 6.24 | 6.40 | 6.39 | 6.26 | 6.25 | | | 6.25 | 6.35 |
| Pyrimidine | $^1B_1(\mathrm{V}; n \to \pi^\star)$ | 4.44 | 4.57 | 4.41 | 4.66 | 4.36 | 4.51 | 4.51 | 4.44 | 4.37 |
| | $^1A_2(\mathrm{V}; n \to \pi^\star)$ | 4.85 | 4.97 | 4.77 | 5.07 | 4.81 | 4.92 | 4.94 | 4.86 | 4.73 |
| | $^1B_2(\mathrm{V}; \pi \to \pi^\star)$ | 5.38 | 5.58 | 5.54 | 5.53 | 5.15 | 5.47 | 5.44 | 5.41 | 5.52 |
| | $^1A_2(\mathrm{V}; n \to \pi^\star)$ | 5.92 | 6.06 | 5.96 | 6.20 | 5.91 | 6.03 | 6.02 | 5.93 | 5.93 |
| | $^1B_1(\mathrm{V}; n \to \pi^\star)$ | 6.26 | 7.22 | 6.25 | 6.54 | 6.26 | 6.34 | 6.36 | 6.26 | 6.22 |
| | $^1B_2(\mathrm{R}; n \to 3s)$ | 6.70 | 6.23 | 6.20 | 6.88 | 6.90 | 6.77 | 6.81 | 6.72 | 6.25 |
| | $^1A_1(\mathrm{V}; \pi \to \pi^\star)$ | 6.88 | 7.07 | 6.84 | 6.97 | | 6.91 | 6.89 | 6.87 | 6.83 |
| | $^3B_1(\mathrm{V}; n \to \pi^\star)$ | 4.09 | 4.31 | 4.07 | 4.25 | 4.02 | | | 4.10 | 4.05 |
| | $^3A_1(\mathrm{V}; \pi \to \pi^\star)$ | *4.51* | 4.91 | 4.77 | 4.39 | 4.11 | | | 4.55 | 4.76 |
| | $^3A_2(\mathrm{V}; n \to \pi^\star)$ | 4.66 | 5.01 | 4.60 | 4.83 | 4.63 | | | 4.66 | 4.58 |
| | $^3B_2(\mathrm{V}; \pi \to \pi^\star)$ | 4.96 | 5.23 | 5.17 | 4.99 | 4.88 | | | 4.96 | 5.14 |
| Pyrrole | $^1A_2(\mathrm{R}; \pi \to 3s)$ | 5.24 | 5.34 | 5.23 | 5.34 | 5.36 | 5.28 | 5.26 | 5.24 | 5.30 |
| | $^1B_1(\mathrm{R}; \pi \to 3p)$ | 6.00 | 6.04 | 5.91 | 6.04 | 6.08 | 6.01 | 6.00 | 5.98 | 5.94 |
| | $^1A_2(\mathrm{R}; \pi \to 3p)$ | 6.00 | 6.04 | 5.96 | 6.09 | 6.15 | 6.04 | 6.03 | 6.01 | 6.03 |
| | $^1B_2(\mathrm{V}; (\pi \to \pi^\star)$ | 6.26 | 6.62 | 6.30 | 6.35 | 6.44 | 6.28 | 6.27 | 6.25 | 6.35 |
| | $^1A_1(\mathrm{V}; \pi \to \pi^\star)$ | 6.30 | 6.64 | 6.47 | 6.51 | | 6.39 | 6.36 | 6.32 | 6.47 |
| | $^1B_2(\mathrm{R}; \pi \to 3p)$ | 6.83 | 7.00 | 6.89 | 6.93 | | 6.85 | 6.85 | 6.83 | 6.91 |
| | $^3B_2(\mathrm{V}; \pi \to \pi^\star)$ | 4.51 | 4.81 | 4.72 | 4.45 | 4.15 | | | 4.53 | 4.71 |
| | $^3A_2(\mathrm{R}; \pi \to 3s)$ | 5.21 | 5.33 | 5.20 | 5.30 | 5.41 | | | 5.21 | 5.27 |
| | $^3A_1(\mathrm{V}; \pi \to \pi^\star)$ | 5.45 | 5.70 | 5.66 | 5.49 | 5.12 | | | 5.46 | 5.62 |
| | $^3B_1(\mathrm{R}; \pi \to 3p)$ | 5.91 | 6.01 | 5.86 | 5.97 | 6.06 | | | 5.92 | 5.89 |
| Tetrazine | $^1B_{3u}(\mathrm{V}; n \to \pi^\star)$ | 2.47 | 2.67 | 2.38 | 2.64 | 2.36 | 2.54 | 2.52 | 2.46 | 2.42 |
| | $^1A_u(\mathrm{V}; n \to \pi^\star)$ | 3.69 | 3.93 | 3.53 | 3.96 | 3.73 | 3.77 | 3.78 | 3.67 | 3.58 |
| | $^1A_g(\mathrm{V}; n, n \to \pi^\star, \pi^\star)$ | *4.61* | | | | | | 6.77 | 6.21 | |
| | $^1B_{1g}(\mathrm{V}; n \to \pi^\star)$ | 4.93 | 5.58 | 5.02 | 5.26 | 4.90 | 5.09 | 5.03 | 4.91 | 5.04 |
| | $^1B_{2u}(\mathrm{V}; \pi \to \pi^\star)$ | 5.21 | 5.40 | 5.31 | 5.37 | 4.92 | 5.31 | 5.26 | 5.23 | 5.31 |

Continued on next page

| Compound | State | TBE | CIS(D) | CC2 | CCSD | STEOM | CC(3) | CCSDT-3 | CC3 | ADC(2) |
|---|---|---|---|---|---|---|---|---|---|---|
| | $^1B_{2g}(\mathrm{V}; n \to \pi^\star)$ | 5.45 | 6.09 | 5.64 | 5.84 | 5.49 | 5.64 | 5.57 | 5.46 | 5.68 |
| | $^1A_u(\mathrm{V}; n \to \pi^\star)$ | 5.53 | 5.64 | 5.56 | 5.77 | 5.50 | 5.63 | | 5.52 | 5.59 |
| | $^1B_{3g}(\mathrm{V}; n, n \to \pi^\star, \pi^\star)$ | *6.15* | | | | | | | 7.62 | |
| | $^1B_{2g}(\mathrm{V}; n \to \pi^\star)$ | 6.12 | 6.08 | 6.18 | 6.66 | | 6.34 | 6.32 | 6.13 | 6.21 |
| | $^1B_{1g}(\mathrm{V}; n \to \pi^\star)$ | 6.91 | 6.39 | 6.95 | 7.32 | | 7.04 | 7.05 | 6.92 | 6.97 |
| | $^3B_{3u}(\mathrm{V}; n \to \pi^\star)$ | 1.85 | 2.13 | 1.81 | 1.96 | 1.70 | | | 1.85 | 1.85 |
| | $^3A_u(\mathrm{V}; n \to \pi^\star)$ | 3.45 | 4.00 | 3.31 | 3.66 | 3.47 | | | 3.44 | 3.35 |
| | $^3B_{1g}(\mathrm{V}; n \to \pi^\star)$ | 4.20 | 4.46 | 4.27 | 4.31 | 3.96 | | | 4.20 | 4.27 |
| | $^3B_{1u}(\mathrm{V}; \pi \to \pi^\star)$ | *4.49* | 4.96 | 4.81 | 4.27 | 3.90 | | | 4.54 | 4.80 |
| | $^3B_{2u}(\mathrm{V}; \pi \to \pi^\star)$ | 4.52 | 4.87 | 4.77 | 4.53 | 4.43 | | | 4.52 | 4.76 |
| | $^3B_{2g}(\mathrm{V}; n \to \pi^\star)$ | 5.04 | 5.47 | 5.15 | 5.23 | 4.91 | | | 5.05 | 5.16 |
| | $^3A_u(\mathrm{V}; n \to \pi^\star)$ | 5.11 | 5.74 | 5.13 | 5.28 | 5.04 | | | 5.11 | 5.16 |
| | $^3B_{3g}(\mathrm{V}; n, n \to \pi^\star, \pi^\star)$ | *5.51* | | | | | | | 7.35 | |
| | $^3B_{1u}(\mathrm{V}; \pi \to \pi^\star)$ | 5.42 | 5.74 | 5.70 | 5.52 | 5.43 | | | 5.42 | 5.67 |
| Thioacetone | $^1A_2(\mathrm{V}; n \to \pi^\star)$ | 2.53 | 2.55 | 2.63 | 2.63 | 2.47 | 2.55 | 2.57 | 2.55 | 2.47 |
| | $^1B_2(\mathrm{R}; n \to 4s)$ | 5.56 | 5.59 | 5.50 | 5.67 | 5.72 | 5.57 | 5.61 | 5.55 | 5.47 |
| | $^1A_1(\mathrm{V}; \pi \to \pi^\star)$ | 5.88 | 6.01 | 6.09 | 6.01 | | 5.90 | 5.93 | 5.90 | 5.87 |
| | $^1B_2(\mathrm{R}; n \to 4p)$ | 6.51 | 6.54 | 6.44 | 6.59 | 6.62 | 6.52 | 6.54 | 6.51 | 6.43 |
| | $^1A_1(\mathrm{R}; n \to 4p)$ | 6.61 | 6.52 | 6.53 | 6.71 | 6.76 | 6.62 | 6.66 | 6.61 | 6.48 |
| | $^3A_2(\mathrm{V}; n \to \pi^\star)$ | 2.33 | 2.30 | 2.33 | 2.35 | 2.25 | | | 2.34 | 2.20 |
| | $^3A_1(\mathrm{V}; \pi \to \pi^\star)$ | 3.45 | 3.60 | 3.59 | 3.66 | 3.22 | | | 3.46 | 3.52 |
| Thiophene | $^1A_1(\mathrm{V}; \pi \to \pi^\star)$ | 5.64 | 5.77 | 5.75 | 5.78 | | 5.69 | 5.69 | 5.65 | 5.72 |
| | $^1B_2(\mathrm{V}; \pi \to \pi^\star)$ | 5.98 | 6.24 | 6.07 | 6.12 | | 6.00 | 5.99 | 5.96 | 6.07 |
| | $^1A_2(\mathrm{R}; \pi \to 3s)$ | 6.14 | 6.18 | 6.07 | 6.22 | 6.18 | 6.17 | 6.15 | 6.14 | 6.15 |
| | $^1B_1(\mathrm{R}; \pi \to 3p)$ | 6.14 | 6.44 | 6.15 | 6.31 | 6.23 | 6.20 | 6.18 | 6.14 | 6.24 |
| | $^1A_2(\mathrm{R}; \pi \to 3p)$ | 6.21 | 6.42 | 6.35 | 6.32 | 6.16 | 6.28 | 6.28 | 6.25 | 6.35 |
| | $^1B_1(\mathrm{R}; \pi \to 3s)$ | 6.49 | 6.49 | 6.48 | 6.56 | 6.52 | 6.52 | 6.52 | 6.50 | 6.51 |
| | $^1B_2(\mathrm{R}; \pi \to 3p)$ | 7.29 | 7.37 | 7.26 | 7.38 | 7.35 | 7.33 | 7.31 | 7.29 | 7.34 |
| | $^1A_1(\mathrm{V}; \pi \to \pi^\star)$ | *7.31* | 7.68 | 7.48 | 7.57 | | 7.46 | 7.42 | 7.35 | 7.51 |
| | $^3B_2(\mathrm{V}; \pi \to \pi^\star)$ | 3.92 | 4.22 | 4.12 | 3.85 | 3.70 | | | 3.94 | 4.11 |
| | $^3A_1(\mathrm{V}; \pi \to \pi^\star)$ | 4.76 | 5.02 | 4.91 | 4.77 | 4.71 | | | 4.77 | 4.86 |
| | $^3B_1(\mathrm{R}; \pi \to 3p)$ | 5.93 | 6.28 | 6.00 | 6.12 | 6.16 | | | 5.95 | 6.09 |
| | $^3A_2(\mathrm{R}; \pi \to 3s)$ | 6.08 | 6.17 | 6.03 | 6.16 | 6.24 | | | 6.09 | 6.11 |
| Thiopropynal | $^1A''(\mathrm{V}; n \to \pi^\star)$ | 2.03 | 2.14 | 2.20 | 2.15 | 2.06 | 2.07 | 2.08 | 2.05 | 2.08 |
| | $^3A''(\mathrm{V}; n \to \pi^\star)$ | 1.80 | 1.83 | 1.84 | 1.83 | 1.79 | | | 1.81 | 1.74 |
| Triazine | $^1A_1''(\mathrm{V}; n \to \pi^\star)$ | 4.72 | 4.59 | 4.64 | 4.92 | 4.62 | 4.77 | 4.80 | 4.73 | 4.58 |
| | $^1A_2''(\mathrm{V}; n \to \pi^\star)$ | 4.75 | 4.86 | 4.75 | 4.99 | 4.76 | 4.82 | 4.82 | 4.74 | 4.69 |
| | $^1E''(\mathrm{V}; n \to \pi^\star)$ | 4.78 | 4.84 | 4.72 | 4.99 | 4.74 | 4.84 | 4.86 | 4.78 | 4.66 |
| | $^1A_2'(\mathrm{V}; \pi \to \pi^\star)$ | 5.75 | 5.83 | 5.89 | 5.91 | 5.45 | 5.85 | 5.82 | 5.78 | 5.83 |

Continued on next page

| Compound | State | TBE | CIS(D) | CC2 | CCSD | STEOM | CC(3) | CCSDT-3 | CC3 | ADC(2) |
|---|---|---|---|---|---|---|---|---|---|---|
| | $^1A_1'$(V; $\pi \rightarrow \pi^\star$) | 7.24 | 7.39 | 7.32 | 7.34 | | 7.28 | 7.27 | 7.24 | 7.18 |
| | $^1E'$(R; $n \rightarrow 3s$) | 7.32 | 7.83 | 6.87 | 7.45 | | 7.37 | 7.41 | 7.35 | 6.89 |
| | $^1E''$(V; $n \rightarrow \pi^\star$) | 7.78 | | 7.71 | 8.13 | | 7.96 | | 7.79 | |
| | $^1E'$(V; $\pi \rightarrow \pi^\star$) | 7.94 | 7.84 | 7.63 | 8.14 | | 7.95 | | 7.92 | 7.65 |
| | $^3A_2''$(V; $n \rightarrow \pi^\star$) | 4.33 | 4.52 | 4.32 | 4.51 | 4.32 | | | 4.33 | 4.29 |
| | $^3E''$(V; $n \rightarrow \pi^\star$) | 4.51 | 4.71 | 4.46 | 4.67 | 4.47 | | | 4.51 | 4.42 |
| | $^3A_1''$(V; $n \rightarrow \pi^\star$) | 4.73 | 4.65 | 4.65 | 4.91 | 4.43 | | | 4.75 | 4.59 |
| | $^3A_1'$(V; $\pi \rightarrow \pi^\star$) | 4.85 | 5.27 | 5.12 | 4.74 | 4.69 | | | 4.88 | 5.10 |
| | $^3E'$(V; $\pi \rightarrow \pi^\star$) | 5.59 | 5.91 | 5.88 | 5.70 | 5.61 | | | 5.61 | 5.82 |
| | $^3A_2'$(V; $(\pi \rightarrow \pi^\star$) | 6.62 | 6.71 | 6.76 | 6.59 | 6.60 | | | 6.63 | 6.63 |

## S4.2 Statistical analysis

Table S41: MSE (in eV) obtained for various subsets of transition energies.

| Method | Singlet | Triplet | Valence | Rydberg | $n \to \pi^\star$ | $\pi \to \pi^\star$ |
|---|---|---|---|---|---|---|
| CIS(D) | 0.10 | 0.24 | 0.24 | -0.05 | 0.19 | 0.28 |
| ADC(2) | -0.04 | 0.07 | 0.06 | -0.13 | -0.04 | 0.14 |
| CC2 | -0.03 | 0.11 | 0.10 | -0.17 | 0.01 | 0.17 |
| STEOM-CCSD | 0.06 | -0.06 | -0.04 | 0.12 | -0.02 | -0.06 |
| CCSD | 0.15 | 0.05 | 0.12 | 0.09 | 0.19 | 0.07 |
| CCSDR(3) | 0.05 | | 0.07 | 0.02 | 0.08 | 0.06 |
| CCSDT-3 | 0.05 | | 0.06 | 0.03 | 0.08 | 0.04 |
| CC3 | 0.00 | 0.01 | 0.01 | 0.00 | 0.00 | 0.01 |
| NEVPT2 | 0.10 | 0.08 | 0.08 | 0.12 | 0.05 | 0.11 |

# S5 Geometries

Below, we provide the cartesian coordinates of the compounds investigated in this study. These are provided in atomic units (bohr) and they have been obtained at the CC3(full)/*aug*-cc-pVTZ level of theory.

## S5.1 Acetone

```
C    0.00000000          0.00000000          0.18807702
C    0.00000000          2.42007545         -1.31764698
C    0.00000000         -2.42007545         -1.31764698
O    0.00000000          0.00000000          2.48269094
H    0.00000000          4.03690733         -0.05185132
H    0.00000000         -4.03690733         -0.05185132
H    1.66061256          2.48420530         -2.53995285
H   -1.66061256          2.48420530         -2.53995285
H    1.66061256         -2.48420530         -2.53995285
H   -1.66061256         -2.48420530         -2.53995285
```

## S5.2 Acrolein

```
C   -1.11645072         -0.68348783          0.00000000
C    1.20647847          0.83714564          0.00000000
C    3.46831059         -0.28872636          0.00000000
O   -3.23666415          0.19187203          0.00000000
H   -0.80613858         -2.74747338          0.00000000
H    0.98699813          2.86613511          0.00000000
H    5.20930864          0.77443560          0.00000000
H    3.60951559         -2.33000749          0.00000000
```

## S5.3 Benzene

| | | | |
|---|---|---|---|
| C | 0.00000000 | 2.63144965 | 0.00000000 |
| C | -2.27890225 | 1.31572483 | 0.00000000 |
| C | -2.27890225 | -1.31572483 | 0.00000000 |
| C | 0.00000000 | -2.63144965 | 0.00000000 |
| C | 2.27890225 | -1.31572483 | 0.00000000 |
| C | 2.27890225 | 1.31572483 | 0.00000000 |
| H | -4.04725813 | 2.33668557 | 0.00000000 |
| H | -4.04725813 | -2.33668557 | 0.00000000 |
| H | -0.00000000 | -4.67337115 | 0.00000000 |
| H | 4.04725813 | -2.33668557 | 0.00000000 |
| H | 4.04725813 | 2.33668557 | 0.00000000 |
| H | 0.00000000 | 4.67337115 | 0.00000000 |

## S5.4 Butadiene

| | | | |
|---|---|---|---|
| C | 1.14656244 | 0.00000000 | 0.75468820 |
| C | -1.14656244 | 0.00000000 | -0.75468820 |
| C | 3.48132647 | 0.00000000 | -0.22482805 |
| C | -3.48132647 | 0.00000000 | 0.22482805 |
| H | 0.90770978 | 0.00000000 | 2.78883925 |
| H | -0.90770978 | 0.00000000 | -2.78883925 |
| H | 3.77525814 | 0.00000000 | -2.24895470 |
| H | -3.77525814 | 0.00000000 | 2.24895470 |
| H | 5.13664967 | 0.00000000 | 0.96861890 |
| H | -5.13664967 | 0.00000000 | -0.96861890 |

## S5.5 Cyanoacetylene

| | | | |
|---|---|---|---|
| C | 0.00000000 | 0.00000000 | -3.59120182 |
| C | 0.00000000 | 0.00000000 | -1.30693904 |
| C | 0.00000000 | 0.00000000 | 1.28880240 |
| N | 0.00000000 | 0.00000000 | 3.48692211 |
| H | 0.00000000 | 0.00000000 | -5.59619886 |

Lowest excited state

| | | | |
|---|---|---|---|
| C | 1.99411175 | 0.00000000 | 2.81781077 |
| C | -0.07304269 | 0.00000000 | 1.33125774 |
| C | -0.63630126 | 0.00000000 | -1.14556678 |
| N | -1.39755756 | 0.00000000 | -3.26154643 |
| H | 1.90749857 | 0.00000000 | 4.87279180 |

## S5.6 Cyanoformaldehyde

| | | | |
|---|---|---|---|
| C | -0.91561483 | 0.00000000 | -1.22522833 |
| C | -0.01092219 | 0.00000000 | 1.39523175 |
| N | 0.64170259 | 0.00000000 | 3.48820325 |
| O | 0.50833684 | 0.00000000 | -3.00337867 |
| H | -2.97202213 | 0.00000000 | -1.42565674 |

## S5.7 Cyanogen

Ground state

| | | | |
|---|---|---|---|
| C | 0.00000000 | 0.00000000 | 1.30401924 |
| C | 0.00000000 | 0.00000000 | -1.30401924 |
| N | 0.00000000 | 0.00000000 | 3.49784121 |
| N | 0.00000000 | 0.00000000 | -3.49784121 |

Lowest excited state

| | | | |
|---|---|---|---|
| C | 0.00000000 | 0.00000000 | 1.22784115 |
| C | 0.00000000 | 0.00000000 | -1.22784115 |
| N | 0.00000000 | 0.00000000 | 3.56462559 |
| N | 0.00000000 | 0.00000000 | -3.56462559 |

## S5.8 Cyclopentadiene

| | | | |
|---|---|---|---|
| C | 0.00000000 | 0.00000000 | -2.33113051 |
| C | 0.00000000 | 2.22209092 | -0.56871188 |
| C | 0.00000000 | -2.22209092 | -0.56871188 |
| C | 0.00000000 | 1.38514451 | 1.83772922 |
| C | 0.00000000 | -1.38514451 | 1.83772922 |
| H | 1.66130504 | 0.00000000 | -3.56414299 |
| H | -1.66130504 | 0.00000000 | -3.56414299 |
| H | 0.00000000 | 4.16550405 | -1.18116624 |
| H | 0.00000000 | -4.16550405 | -1.18116624 |
| H | 0.00000000 | 2.54514584 | 3.51352303 |
| H | 0.00000000 | -2.54514584 | 3.51352303 |

## S5.9 Cyclopropenone

| | | | |
|---|---|---|---|
| C | 0.00000000 | 1.27491826 | -1.86930519 |
| C | 0.00000000 | -1.27491826 | -1.86930519 |
| C | 0.00000000 | 0.00000000 | 0.51814554 |
| O | 0.00000000 | 0.00000000 | 2.79326776 |
| H | 0.00000000 | 2.92791371 | -3.05679837 |
| H | 0.00000000 | -2.92791371 | -3.05679837 |

## S5.10 Cyclopropenethione

| | | | |
|---|---|---|---|
| C | 0.00000000 | 1.26230744 | -2.86571925 |
| C | 0.00000000 | -1.26230744 | -2.86571925 |
| C | 0.00000000 | 0.00000000 | -0.49233236 |
| S | 0.00000000 | 0.00000000 | 2.57821680 |
| H | 0.00000000 | 2.97773331 | -3.95114059 |
| H | 0.00000000 | -2.97773331 | -3.95114059 |

## S5.11 Diacetylene

| | | | |
|---|---|---|---|
| C | 0.00000000 | 0.00000000 | 1.29447700 |
| C | 0.00000000 | 0.00000000 | -1.29447700 |
| C | 0.00000000 | 0.00000000 | 3.58448429 |
| C | 0.00000000 | 0.00000000 | -3.58448429 |
| H | 0.00000000 | 0.00000000 | 5.58943003 |
| H | 0.00000000 | 0.00000000 | -5.58943003 |

## S5.12 Furan

| | | | |
|---|---|---|---|
| C | 0.00000000 | 2.06365826 | -0.60051250 |
| C | 0.00000000 | -2.06365826 | -0.60051250 |
| C | 0.00000000 | 1.35348578 | 1.86336416 |
| C | 0.00000000 | -1.35348578 | 1.86336416 |
| O | 0.00000000 | 0.00000000 | -2.13945332 |
| H | 0.00000000 | 3.86337287 | -1.53765695 |
| H | 0.00000000 | -3.86337287 | -1.53765695 |
| H | 0.00000000 | 2.59168789 | 3.47168051 |
| H | 0.00000000 | -2.59168789 | 3.47168051 |

## S5.13 Glyoxal

| | | | |
|---|---|---|---|
| C | 1.21360282 | 0.75840215 | 0.00000000 |
| C | -1.21360282 | -0.75840215 | 0.00000000 |
| O | 3.25581408 | -0.26453186 | 0.00000000 |
| O | -3.25581408 | 0.26453186 | 0.00000000 |
| H | 0.96135276 | 2.81883243 | 0.00000000 |
| H | -0.96135276 | -2.81883243 | 0.00000000 |

## S5.14 Imidazole

| | | | |
|---|---|---|---|
| C | 0.41662795 | 2.06006259 | 0.00000000 |
| C | -1.52618386 | -1.62343163 | 0.00000000 |
| C | 1.04160471 | -1.93007427 | 0.00000000 |
| N | -1.90345764 | 0.94914956 | 0.00000000 |
| N | 2.24215443 | 0.38083431 | 0.00000000 |
| H | 0.65501634 | 4.07748278 | 0.00000000 |
| H | -3.57500545 | 1.84103166 | 0.00000000 |
| H | -3.06363894 | -2.94559167 | 0.00000000 |
| H | 2.08673940 | -3.67001102 | 0.00000000 |

## S5.15 Isobutene

| | | | |
|---|---|---|---|
| C | 0.00000000 | 0.00000000 | 2.70790758 |
| C | 0.00000000 | 0.00000000 | 0.18431282 |
| C | 0.00000000 | 2.39894572 | -1.32482735 |
| C | 0.00000000 | -2.39894572 | -1.32482735 |
| H | 0.00000000 | 1.74848405 | 3.76691310 |
| H | 0.00000000 | -1.74848405 | 3.76691310 |
| H | 0.00000000 | 4.05897160 | -0.10582007 |
| H | 0.00000000 | -4.05897160 | -0.10582007 |
| H | 1.66026992 | 2.48337908 | -2.55086178 |
| H | -1.66026992 | 2.48337908 | -2.55086178 |
| H | 1.66026992 | -2.48337908 | -2.55086178 |
| H | -1.66026992 | -2.48337908 | -2.55086178 |

## S5.16 Methylenecyclopropene

| | | | |
|---|---|---|---|
| C | 0.00000000 | 0.00000000 | 0.53512883 |
| C | 0.00000000 | 0.00000000 | 3.04739824 |
| C | 0.00000000 | 1.25042956 | -1.88571561 |
| C | 0.00000000 | -1.25042956 | -1.88571561 |
| H | 0.00000000 | 2.96887531 | -2.96270271 |
| H | 0.00000000 | -2.96887531 | -2.96270271 |
| H | 0.00000000 | 1.75335023 | 4.08608382 |
| H | 0.00000000 | -1.75335023 | 4.08608382 |

## S5.17 Propynal

| | | | |
|---|---|---|---|
| C | -0.78051115 | 0.00000000 | -1.38900384 |
| C | -0.17873562 | 0.00000000 | 1.27825868 |
| C | 0.23763714 | 0.00000000 | 3.52644798 |
| O | 0.80143996 | 0.00000000 | -3.04628328 |
| H | -2.80713069 | 0.00000000 | -1.82768750 |
| H | 0.64026209 | 0.00000000 | 5.48853193 |

## S5.18 Pyrazine

| | | | |
|---|---|---|---|
| C | 0.00000000 | 2.13188686 | 1.31510863 |
| C | 0.00000000 | -2.13188686 | 1.31510863 |
| C | 0.00000000 | 2.13188686 | -1.31510863 |
| C | 0.00000000 | -2.13188686 | -1.31510863 |
| N | 0.00000000 | 0.00000000 | 2.66620111 |
| N | 0.00000000 | 0.00000000 | -2.66620111 |
| H | 0.00000000 | 3.88751412 | 2.35234226 |
| H | 0.00000000 | -3.88751412 | 2.35234226 |
| H | 0.00000000 | 3.88751412 | -2.35234226 |
| H | 0.00000000 | -3.88751412 | -2.35234226 |

## S5.19 Pyridazine

| | | | |
|---|---|---|---|
| C | 0.00000000 | 1.30150855 | -2.31552865 |
| C | 0.00000000 | -1.30150855 | -2.31552865 |
| C | 0.00000000 | 2.49271907 | 0.03513416 |
| C | 0.00000000 | -2.49271907 | 0.03513416 |
| N | 0.00000000 | 1.26228251 | 2.23104685 |
| N | 0.00000000 | -1.26228251 | 2.23104685 |
| H | 0.00000000 | 4.52804172 | 0.19299731 |
| H | 0.00000000 | -4.52804172 | 0.19299731 |
| H | 0.00000000 | 2.39011496 | -4.03967703 |
| H | 0.00000000 | -2.39011496 | -4.03967703 |

## S5.20 Pyridine

| | | | |
|---|---|---|---|
| C | 0.00000000 | 0.00000000 | -2.66451139 |
| C | 0.00000000 | 2.25494985 | -1.32069889 |
| C | 0.00000000 | -2.25494985 | -1.32069889 |
| C | 0.00000000 | 2.15398594 | 1.30669632 |
| C | 0.00000000 | -2.15398594 | 1.30669632 |
| N | 0.00000000 | 0.00000000 | 2.62778932 |
| H | 0.00000000 | 0.00000000 | -4.70641516 |
| H | 0.00000000 | 4.05768507 | -2.27625442 |
| H | 0.00000000 | -4.05768507 | -2.27625442 |
| H | 0.00000000 | 3.88059079 | 2.40341581 |
| H | 0.00000000 | -3.88059079 | 2.40341581 |

## S5.21 Pyrimidine

| | | | |
|---|---|---|---|
| C | 0.00000000 | 0.00000000 | 2.41518350 |
| C | 0.00000000 | -0.00000000 | -2.60410885 |
| C | 0.00000000 | 2.23272561 | -1.22869402 |
| C | 0.00000000 | -2.23272561 | -1.22869402 |
| N | 0.00000000 | 2.26214196 | 1.29619742 |
| N | 0.00000000 | -2.26214196 | 1.29619742 |
| H | 0.00000000 | 0.00000000 | 4.45780256 |
| H | 0.00000000 | 0.00000000 | -4.64120942 |
| H | 0.00000000 | 4.05149341 | -2.16351748 |
| H | 0.00000000 | -4.05149341 | -2.16351748 |

## S5.22 Pyrrole

| | | | |
|---|---|---|---|
| C | 0.00000000 | 2.11924634 | 0.62676569 |
| C | 0.00000000 | -2.11924634 | 0.62676569 |
| C | 0.00000000 | 1.34568862 | -1.85506908 |
| C | 0.00000000 | -1.34568862 | -1.85506908 |
| N | 0.00000000 | 0.00000000 | 2.10934391 |
| H | 0.00000000 | 0.00000000 | 4.00257355 |
| H | 0.00000000 | 3.97648410 | 1.44830201 |
| H | 0.00000000 | -3.97648410 | 1.44830201 |
| H | 0.00000000 | 2.56726559 | -3.47837232 |
| H | 0.00000000 | -2.56726559 | -3.47837232 |

## S5.23 Tetrazine

| | | | |
|---|---|---|---|
| C | 0.00000000 | 0.00000000 | 2.38208164 |
| C | 0.00000000 | 0.00000000 | -2.38208164 |
| N | 2.25673244 | 0.00000000 | 1.24973261 |
| N | -2.25673244 | 0.00000000 | 1.24973261 |
| N | 2.25673244 | 0.00000000 | -1.24973261 |
| N | -2.25673244 | 0.00000000 | -1.24973261 |
| H | 0.00000000 | 0.00000000 | 4.41850901 |
| H | 0.00000000 | 0.00000000 | -4.41850901 |

## S5.24 Thioacetone

| | | | |
|---|---|---|---|
| C | 0.00000000 | 0.00000000 | 0.68476030 |
| C | 0.00000000 | 2.38541696 | 2.20685096 |
| C | 0.00000000 | -2.38541696 | 2.20685096 |
| S | 0.00000000 | 0.00000000 | -2.39920303 |
| H | 0.00000000 | 4.04609254 | 1.00090614 |
| H | 0.00000000 | -4.04609254 | 1.00090614 |
| H | 1.65894780 | 2.42602225 | 3.43712000 |
| H | -1.65894780 | 2.42602225 | 3.43712000 |
| H | 1.65894780 | -2.42602225 | 3.43712000 |
| H | -1.65894780 | -2.42602225 | 3.43712000 |

## S5.25 Thiophene

| | | | |
|---|---|---|---|
| C | 0.00000000 | 2.33342542 | -0.09858421 |
| C | 0.00000000 | -2.33342542 | -0.09858421 |
| C | 0.00000000 | 1.34371718 | -2.48297725 |
| C | 0.00000000 | -1.34371718 | -2.48297725 |
| S | 0.00000000 | 0.00000000 | 2.17250692 |
| H | 0.00000000 | 4.29028016 | 0.44577296 |
| H | 0.00000000 | -4.29028016 | 0.44577296 |
| H | 0.00000000 | 2.48760051 | -4.16768392 |
| H | 0.00000000 | -2.48760051 | -4.16768392 |

## S5.26 Thiopropynal

| | | | |
|---|---|---|---|
| C | -0.00382924 | 0.00000000 | -1.25249909 |
| C | -2.27832423 | 0.00000000 | 0.15152736 |
| C | -4.26309583 | 0.00000000 | 1.29548793 |
| S | 2.81920288 | 0.00000000 | -0.00828974 |
| H | -0.23056990 | 0.00000000 | -3.28862183 |
| H | -5.97712967 | 0.00000000 | 2.33206931 |

## S5.27 Triazine

| | | | |
|---|---|---|---|
| C | 0.00000000 | -2.11414732 | -1.22060353 |
| C | 0.00000000 | 0.00000000 | 2.44120705 |
| C | 0.00000000 | 2.11414732 | -1.22060353 |
| N | 0.00000000 | -2.24624733 | 1.29687150 |
| N | 0.00000000 | 2.24624733 | 1.29687150 |
| N | 0.00000000 | 0.00000000 | -2.59374300 |
| H | 0.00000000 | 3.88296710 | -2.24183210 |
| H | 0.00000000 | -3.88296710 | -2.24183210 |
| H | 0.00000000 | 0.00000000 | 4.48366420 |
